# Supplementary material for: Autonomic Management in a Distributed Storage System
Source: arXiv:1007.0328 source file (2010-07-02)
Supplement: Supplementary file 1 [file p2p.tex]

GAMF was used in experiments in which autonomic management was applied to P2P nodes ({\it StAChord}). 
This description focuses on how autonomic management was applied to the target system ({\it StAChord}). 
The source code of StAChord was available. This allowed the integration of event generators and effectors in StAChord.
 
The objective of the experiment mentioned above was to manage the scheduling of StAChord's housekeeping operations. The housekeeping mechanism is implemented as a \emph{Java Thread} which constantly carries out maintenance operations after sleeping for a specific interval. It was recorded when a housekeeping operation was carried out unnecessarily, and when the state maintained by the housekeeping operation was not accurate and caused operations to fail. This was achieved by an event generator which was internally (meaning in the same address space) triggered after every maintenance operation execution which had no effect on the maintained state. The same event generator was triggered when any operation failed due to an inaccurate state. To adapt the scheduling of the housekeeping, an effector was implemented which interrupted the thread when triggered, and another effector which changed the interval. 

GAMF operated here in the same address space as a StAChord node. An advantage of this approach is that potential communication costs between different address spaces can be avoided. Additionally, the management code can be maintained in the same code base as the target system.
