# Supplementary material for: Autonomic Management in a Distributed Storage System
Source: arXiv:1007.0328 source file (2010-07-02)
Supplement: Supplementary file 2 [file p2p_main_results_reports_holistic.tex]

\newpage

\subsection{\label{sec:WL1_NB1}Synthetic Light Weight Workload Network with Low Membership Churn}

\begin{figure}[htpb]

	\centerline{{\footnotesize \resizebox{70mm}{!}{\includegraphics{./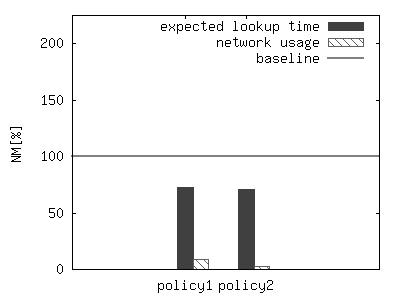}}}}

	\caption{\label{fig:Holistic Synthetic Light Weight Workload Network with Low Membership Churn user-level metrics} mean normalised monitored ULMs averaged over 3 repetitions (NM)}

\end{figure}

\begin{table}[htpb]

	\begin{center}

	{\footnotesize

		\begin{tabular}[t]{|l|r|r|r|r|r|r|}

		\hline user-level metric & unit &  $\mu$ & $\sigma$ & q1 & q2 & q3\\\hline

		expected lookup time & [ms] &720 & NA & NA & NA & NA\\\hline

		network usage& [MB] & 599 & 8 & 590 & 603 & 606\\\hline

		workload lookup time (sec. ULM)& [ms] & 720 & 207 & 516 & 777 & 857\\\hline

		workload error rate (sec. ULM) & [\%] & 0 & 0 & 0 & 0 & 0 \\\hline

		\end{tabular}

		\caption{{\footnotesize ULM distributions, measured with unmanaged nodes. 

}}

		\begin{tabular}[t]{|l|r|r|r|r|r|r|}

		\hline user-level metric & unit &  $\mu$ & $\sigma$ & q1 & q2 & q3\\\hline

		expected lookup time & [ms] &522 & NA & NA & NA & NA\\\hline

		network usage& [MB] & 54 & 0 & 54 & 54 & 54\\\hline

		workload lookup time (sec. ULM)& [ms] & 522 & 145 & 406 & 535 & 607\\\hline

		workload error rate (sec. ULM) & [\%] & 0 & 0 & 0 & 0 & 0 \\\hline

		\end{tabular}

		\caption{{\footnotesize ULM distributions, measured with managed nodes (policy 1). 

}}

		\begin{tabular}[t]{|l|r|r|r|r|r|r|}

		\hline user-level metric & unit &  $\mu$ & $\sigma$ & q1 & q2 & q3\\\hline

		expected lookup time & [ms] &507 & NA & NA & NA & NA\\\hline

		network usage& [MB] & 17 & 0 & 17 & 17 & 17\\\hline

		workload lookup time (sec. ULM)& [ms] & 507 & 121 & 425 & 567 & 606\\\hline

		workload error rate (sec. ULM) & [\%] & 0 & 0 & 0 & 0 & 0 \\\hline

		\end{tabular}

		\caption{{\footnotesize ULM distributions, measured with managed nodes (policy 2). 

}}

	}

	\end{center}

\end{table}

\newpage

\subsection{\label{sec:WL1_NB2}Synthetic Light Weight Workload Network with High Membership Churn}

\begin{figure}[htpb]

	\centerline{{\footnotesize \resizebox{70mm}{!}{\includegraphics{./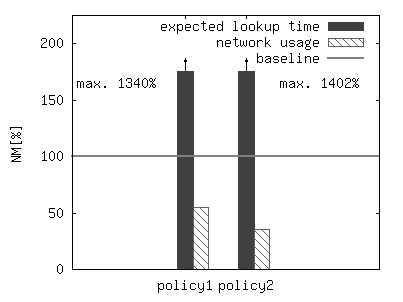}}}}

	\caption{\label{fig:Holistic Synthetic Light Weight Workload Network with High Membership Churn user-level metrics} mean normalised monitored ULMs averaged over 3 repetitions (NM)}

\end{figure}

\begin{table}[htpb]

	\begin{center}

	{\footnotesize

		\begin{tabular}[t]{|l|r|r|r|r|r|r|}

		\hline user-level metric & unit &  $\mu$ & $\sigma$ & q1 & q2 & q3\\\hline

		expected lookup time & [ms] &566 & NA & NA & NA & NA\\\hline

		network usage& [MB] & 327 & 28 & 296 & 333 & 352\\\hline

		workload lookup time (sec. ULM)& [ms] & 562 & 296 & 398 & 551 & 637\\\hline

		time until lookup failed (sec. ULM)& [ms] & 11 & 4 & 8 & 11 & 13\\\hline

		workload error rate (sec. ULM)& [\%] & 7 & 12 & 0 & 0 & 20\\\hline

		\end{tabular}

		\caption{{\footnotesize ULM distributions, measured with unmanaged nodes. 

}}

		\begin{tabular}[t]{|l|r|r|r|r|r|r|}

		\hline user-level metric & unit &  $\mu$ & $\sigma$ & q1 & q2 & q3\\\hline

		expected lookup time & [ms] &7584 & NA & NA & NA & NA\\\hline

		network usage& [MB] & 179 & 11 & 167 & 183 & 188\\\hline

		workload lookup time (sec. ULM)& [ms] & 457 & 166 & 386 & 482 & 544\\\hline

		time until lookup failed (sec. ULM)& [ms] & 16493 & 49431 & 13 & 17 & 20\\\hline

		workload error rate (sec. ULM)& [\%] & 30 & 10 & 20 & 30 & 40\\\hline

		\end{tabular}

		\caption{{\footnotesize ULM distributions, measured with managed nodes (policy 1). 

}}

		\begin{tabular}[t]{|l|r|r|r|r|r|r|}

		\hline user-level metric & unit &  $\mu$ & $\sigma$ & q1 & q2 & q3\\\hline

		expected lookup time & [ms] &7930 & NA & NA & NA & NA\\\hline

		network usage& [MB] & 116 & 5 & 113 & 113 & 121\\\hline

		workload lookup time (sec. ULM)& [ms] & 459 & 265 & 311 & 428 & 527\\\hline

		time until lookup failed (sec. ULM)& [ms] & 12555 & 41412 & 13 & 47 & 49\\\hline

		workload error rate (sec. ULM)& [\%] & 37 & 12 & 30 & 30 & 50\\\hline

		\end{tabular}

		\caption{{\footnotesize ULM distributions, measured with managed nodes (policy 2). 

}}

	}

	\end{center}

\end{table}

\newpage

\subsection{\label{sec:WL1_NB3}Synthetic Light Weight Workload Network with Locally Varying Membership Churn}

\begin{figure}[htpb]

	\centerline{{\footnotesize \resizebox{70mm}{!}{\includegraphics{./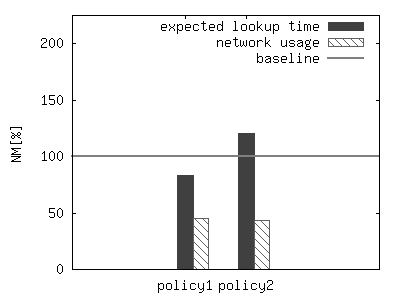}}}}

	\caption{\label{fig:Holistic Synthetic Light Weight Workload Network with Locally Varying Membership Churn user-level metrics} mean normalised monitored ULMs averaged over 3 repetitions (NM)}

\end{figure}

\begin{table}[htpb]

	\begin{center}

	{\footnotesize

		\begin{tabular}[t]{|l|r|r|r|r|r|r|}

		\hline user-level metric & unit &  $\mu$ & $\sigma$ & q1 & q2 & q3\\\hline

		expected lookup time & [ms] &689 & NA & NA & NA & NA\\\hline

		network usage& [MB] & 396 & 8 & 387 & 399 & 401\\\hline

		workload lookup time (sec. ULM)& [ms] & 689 & 248 & 550 & 708 & 830\\\hline

		workload error rate (sec. ULM) & [\%] & 0 & 0 & 0 & 0 & 0 \\\hline

		\end{tabular}

		\caption{{\footnotesize ULM distributions, measured with unmanaged nodes. 

}}

		\begin{tabular}[t]{|l|r|r|r|r|r|r|}

		\hline user-level metric & unit &  $\mu$ & $\sigma$ & q1 & q2 & q3\\\hline

		expected lookup time & [ms] &614 & NA & NA & NA & NA\\\hline

		network usage& [MB] & 180 & 1 & 179 & 179 & 181\\\hline

		workload lookup time (sec. ULM)& [ms] & 575 & 224 & 422 & 612 & 712\\\hline

		time until lookup failed (sec. ULM)& [ms] & 186 & 133 & 55 & 201 & 301\\\hline

		workload error rate (sec. ULM)& [\%] & 13 & 6 & 10 & 10 & 20\\\hline

		\end{tabular}

		\caption{{\footnotesize ULM distributions, measured with managed nodes (policy 1). 

}}

		\begin{tabular}[t]{|l|r|r|r|r|r|r|}

		\hline user-level metric & unit &  $\mu$ & $\sigma$ & q1 & q2 & q3\\\hline

		expected lookup time & [ms] &856 & NA & NA & NA & NA\\\hline

		network usage& [MB] & 173 & 37 & 132 & 187 & 201\\\hline

		workload lookup time (sec. ULM)& [ms] & 831 & 574 & 448 & 701 & 947\\\hline

		time until lookup failed (sec. ULM)& [ms] & 56 & 93 & 9 & 11 & 149\\\hline

		workload error rate (sec. ULM)& [\%] & 13 & 6 & 10 & 10 & 20\\\hline

		\end{tabular}

		\caption{{\footnotesize ULM distributions, measured with managed nodes (policy 2). 

}}

	}

	\end{center}

\end{table}

\newpage

\subsection{\label{sec:WL1_NB4}Synthetic Light Weight Workload Network with Temporal Varying Membership Churn}

\begin{figure}[htpb]

	\centerline{{\footnotesize \resizebox{70mm}{!}{\includegraphics{./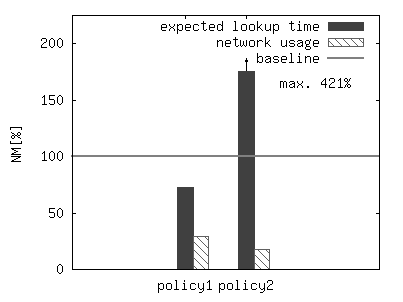}}}}

	\caption{\label{fig:Holistic Synthetic Light Weight Workload Network with Temporal Varying Membership Churn user-level metrics} mean normalised monitored ULMs averaged over 3 repetitions (NM)}

\end{figure}

\begin{table}[htpb]

	\begin{center}

	{\footnotesize

		\begin{tabular}[t]{|l|r|r|r|r|r|r|}

		\hline user-level metric & unit &  $\mu$ & $\sigma$ & q1 & q2 & q3\\\hline

		expected lookup time & [ms] &715 & NA & NA & NA & NA\\\hline

		network usage& [MB] & 437 & 26 & 408 & 446 & 458\\\hline

		workload lookup time (sec. ULM)& [ms] & 643 & 232 & 463 & 602 & 871\\\hline

		time until lookup failed (sec. ULM)& [ms] & 397 & 767 & 13 & 14 & 1165\\\hline

		workload error rate (sec. ULM)& [\%] & 13 & 6 & 10 & 10 & 20\\\hline

		\end{tabular}

		\caption{{\footnotesize ULM distributions, measured with unmanaged nodes. 

}}

		\begin{tabular}[t]{|l|r|r|r|r|r|r|}

		\hline user-level metric & unit &  $\mu$ & $\sigma$ & q1 & q2 & q3\\\hline

		expected lookup time & [ms] &525 & NA & NA & NA & NA\\\hline

		network usage& [MB] & 128 & 15 & 116 & 124 & 145\\\hline

		workload lookup time (sec. ULM)& [ms] & 518 & 152 & 441 & 466 & 604\\\hline

		time until lookup failed (sec. ULM)& [ms] & 12 & 0 & 12 & 12 & 12\\\hline

		workload error rate (sec. ULM)& [\%] & 10 & 0 & 10 & 10 & 10\\\hline

		\end{tabular}

		\caption{{\footnotesize ULM distributions, measured with managed nodes (policy 1). 

}}

		\begin{tabular}[t]{|l|r|r|r|r|r|r|}

		\hline user-level metric & unit &  $\mu$ & $\sigma$ & q1 & q2 & q3\\\hline

		expected lookup time & [ms] &3010 & NA & NA & NA & NA\\\hline

		network usage& [MB] & 78 & 25 & 61 & 67 & 107\\\hline

		workload lookup time (sec. ULM)& [ms] & 629 & 503 & 311 & 466 & 680\\\hline

		time until lookup failed (sec. ULM)& [ms] & 15855 & 18374 & 9 & 14820 & 32735\\\hline

		workload error rate (sec. ULM)& [\%] & 13 & 6 & 10 & 10 & 20\\\hline

		\end{tabular}

		\caption{{\footnotesize ULM distributions, measured with managed nodes (policy 2). 

}}

	}

	\end{center}

\end{table}

\newpage

\subsection{\label{sec:WL2_NB1}Synthetic Heavy Weight Workload Network with Low Membership Churn}

\begin{figure}[htpb]

	\centerline{{\footnotesize \resizebox{70mm}{!}{\includegraphics{./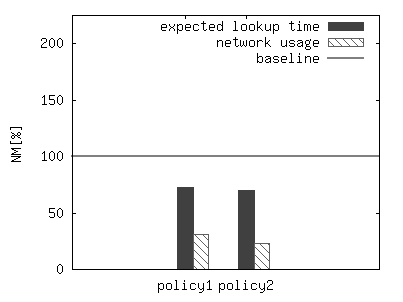}}}}

	\caption{\label{fig:Holistic Synthetic Heavy Weight Workload Network with Low Membership Churn user-level metrics} mean normalised monitored ULMs averaged over 3 repetitions (NM)}

\end{figure}

\begin{table}[htpb]

	\begin{center}

	{\footnotesize

		\begin{tabular}[t]{|l|r|r|r|r|r|r|}

		\hline user-level metric & unit &  $\mu$ & $\sigma$ & q1 & q2 & q3\\\hline

		expected lookup time & [ms] &613 & NA & NA & NA & NA\\\hline

		network usage& [MB] & 891 & 1 & 890 & 891 & 892\\\hline

		workload lookup time (sec. ULM)& [ms] & 613 & 228 & 444 & 615 & 774\\\hline

		workload error rate (sec. ULM) & [\%] & 0 & 0 & 0 & 0 & 0 \\\hline

		\end{tabular}

		\caption{{\footnotesize ULM distributions, measured with unmanaged nodes. 

}}

		\begin{tabular}[t]{|l|r|r|r|r|r|r|}

		\hline user-level metric & unit &  $\mu$ & $\sigma$ & q1 & q2 & q3\\\hline

		expected lookup time & [ms] &445 & NA & NA & NA & NA\\\hline

		network usage& [MB] & 194 & 1 & 193 & 194 & 194\\\hline

		workload lookup time (sec. ULM)& [ms] & 445 & 152 & 354 & 445 & 552\\\hline

		workload error rate (sec. ULM) & [\%] & 0 & 0 & 0 & 0 & 0 \\\hline

		\end{tabular}

		\caption{{\footnotesize ULM distributions, measured with managed nodes (policy 1). 

}}

		\begin{tabular}[t]{|l|r|r|r|r|r|r|}

		\hline user-level metric & unit &  $\mu$ & $\sigma$ & q1 & q2 & q3\\\hline

		expected lookup time & [ms] &428 & NA & NA & NA & NA\\\hline

		network usage& [MB] & 142 & 1 & 141 & 141 & 143\\\hline

		workload lookup time (sec. ULM)& [ms] & 428 & 142 & 322 & 419 & 549\\\hline

		time until lookup failed (sec. ULM)& [ms] & 206 & 0 & 206 & 206 & 206\\\hline

		workload error rate (sec. ULM)& [\%] & 0 & 0 & 0 & 0 & 0\\\hline

		\end{tabular}

		\caption{{\footnotesize ULM distributions, measured with managed nodes (policy 2). 

}}

	}

	\end{center}

\end{table}

\newpage

\subsection{\label{sec:WL2_NB2}Synthetic Heavy Weight Workload Network with High Membership Churn}

\begin{figure}[htpb]

	\centerline{{\footnotesize \resizebox{70mm}{!}{\includegraphics{./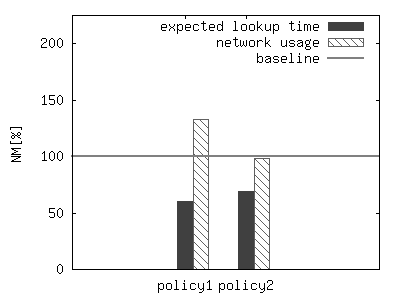}}}}

	\caption{\label{fig:Holistic Synthetic Heavy Weight Workload Network with High Membership Churn user-level metrics} mean normalised monitored ULMs averaged over 3 repetitions (NM)}

\end{figure}

\begin{table}[htpb]

	\begin{center}

	{\footnotesize

		\begin{tabular}[t]{|l|r|r|r|r|r|r|}

		\hline user-level metric & unit &  $\mu$ & $\sigma$ & q1 & q2 & q3\\\hline

		expected lookup time & [ms] &772 & NA & NA & NA & NA\\\hline

		network usage& [MB] & 230 & 199 & 109 & 121 & 460\\\hline

		workload lookup time (sec. ULM)& [ms] & 590 & 256 & 406 & 623 & 750\\\hline

		time until lookup failed (sec. ULM)& [ms] & 152 & 1181 & 67 & 99 & 110\\\hline

		workload error rate (sec. ULM)& [\%] & 34 & 34 & 3 & 29 & 70\\\hline

		\end{tabular}

		\caption{{\footnotesize ULM distributions, measured with unmanaged nodes. 

}}

		\begin{tabular}[t]{|l|r|r|r|r|r|r|}

		\hline user-level metric & unit &  $\mu$ & $\sigma$ & q1 & q2 & q3\\\hline

		expected lookup time & [ms] &443 & NA & NA & NA & NA\\\hline

		network usage& [MB] & 296 & 3 & 293 & 295 & 299\\\hline

		workload lookup time (sec. ULM)& [ms] & 434 & 208 & 278 & 412 & 558\\\hline

		time until lookup failed (sec. ULM)& [ms] & 196 & 160 & 86 & 185 & 263\\\hline

		workload error rate (sec. ULM)& [\%] & 4 & 0 & 4 & 4 & 4\\\hline

		\end{tabular}

		\caption{{\footnotesize ULM distributions, measured with managed nodes (policy 1). 

}}

		\begin{tabular}[t]{|l|r|r|r|r|r|r|}

		\hline user-level metric & unit &  $\mu$ & $\sigma$ & q1 & q2 & q3\\\hline

		expected lookup time & [ms] &474 & NA & NA & NA & NA\\\hline

		network usage& [MB] & 218 & 21 & 203 & 209 & 242\\\hline

		workload lookup time (sec. ULM)& [ms] & 409 & 198 & 275 & 389 & 523\\\hline

		time until lookup failed (sec. ULM)& [ms] & 482 & 6545 & 142 & 185 & 251\\\hline

		workload error rate (sec. ULM)& [\%] & 11 & 4 & 8 & 9 & 15\\\hline

		\end{tabular}

		\caption{{\footnotesize ULM distributions, measured with managed nodes (policy 2). 

}}

	}

	\end{center}

\end{table}

\newpage

\subsection{\label{sec:WL2_NB3}Synthetic Heavy Weight Workload Network with Locally Varying Membership Churn}

\begin{figure}[htpb]

	\centerline{{\footnotesize \resizebox{70mm}{!}{\includegraphics{./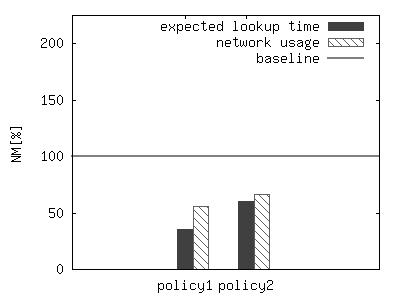}}}}

	\caption{\label{fig:Holistic Synthetic Heavy Weight Workload Network with Locally Varying Membership Churn user-level metrics} mean normalised monitored ULMs averaged over 3 repetitions (NM)}

\end{figure}

\begin{table}[htpb]

	\begin{center}

	{\footnotesize

		\begin{tabular}[t]{|l|r|r|r|r|r|r|}

		\hline user-level metric & unit &  $\mu$ & $\sigma$ & q1 & q2 & q3\\\hline

		expected lookup time & [ms] &1370 & NA & NA & NA & NA\\\hline

		network usage& [MB] & 529 & 101 & 412 & 587 & 587\\\hline

		workload lookup time (sec. ULM)& [ms] & 840 & 657 & 416 & 647 & 944\\\hline

		time until lookup failed (sec. ULM)& [ms] & 2447 & 17738 & 74 & 166 & 525\\\hline

		workload error rate (sec. ULM)& [\%] & 17 & 14 & 1 & 19 & 30\\\hline

		\end{tabular}

		\caption{{\footnotesize ULM distributions, measured with unmanaged nodes. 

}}

		\begin{tabular}[t]{|l|r|r|r|r|r|r|}

		\hline user-level metric & unit &  $\mu$ & $\sigma$ & q1 & q2 & q3\\\hline

		expected lookup time & [ms] &491 & NA & NA & NA & NA\\\hline

		network usage& [MB] & 296 & 9 & 288 & 294 & 305\\\hline

		workload lookup time (sec. ULM)& [ms] & 444 & 204 & 279 & 421 & 589\\\hline

		time until lookup failed (sec. ULM)& [ms] & 871 & 12153 & 143 & 186 & 236\\\hline

		workload error rate (sec. ULM)& [\%] & 5 & 1 & 5 & 5 & 6\\\hline

		\end{tabular}

		\caption{{\footnotesize ULM distributions, measured with managed nodes (policy 1). 

}}

		\begin{tabular}[t]{|l|r|r|r|r|r|r|}

		\hline user-level metric & unit &  $\mu$ & $\sigma$ & q1 & q2 & q3\\\hline

		expected lookup time & [ms] &825 & NA & NA & NA & NA\\\hline

		network usage& [MB] & 353 & 66 & 309 & 322 & 429\\\hline

		workload lookup time (sec. ULM)& [ms] & 541 & 438 & 283 & 444 & 662\\\hline

		time until lookup failed (sec. ULM)& [ms] & 1527 & 15181 & 141 & 186 & 243\\\hline

		workload error rate (sec. ULM)& [\%] & 16 & 9 & 10 & 11 & 25\\\hline

		\end{tabular}

		\caption{{\footnotesize ULM distributions, measured with managed nodes (policy 2). 

}}

	}

	\end{center}

\end{table}

\newpage

\subsection{\label{sec:WL2_NB4}Synthetic Heavy Weight Workload Network with Temporal Varying Membership Churn}

\begin{figure}[htpb]

	\centerline{{\footnotesize \resizebox{70mm}{!}{\includegraphics{./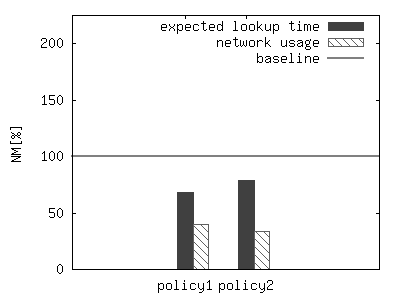}}}}

	\caption{\label{fig:Holistic Synthetic Heavy Weight Workload Network with Temporal Varying Membership Churn user-level metrics} mean normalised monitored ULMs averaged over 3 repetitions (NM)}

\end{figure}

\begin{table}[htpb]

	\begin{center}

	{\footnotesize

		\begin{tabular}[t]{|l|r|r|r|r|r|r|}

		\hline user-level metric & unit &  $\mu$ & $\sigma$ & q1 & q2 & q3\\\hline

		expected lookup time & [ms] &655 & NA & NA & NA & NA\\\hline

		network usage& [MB] & 629 & 84 & 532 & 676 & 678\\\hline

		workload lookup time (sec. ULM)& [ms] & 622 & 408 & 409 & 570 & 739\\\hline

		time until lookup failed (sec. ULM)& [ms] & 196 & 745 & 97 & 105 & 128\\\hline

		workload error rate (sec. ULM)& [\%] & 11 & 17 & 1 & 1 & 31\\\hline

		\end{tabular}

		\caption{{\footnotesize ULM distributions, measured with unmanaged nodes. 

}}

		\begin{tabular}[t]{|l|r|r|r|r|r|r|}

		\hline user-level metric & unit &  $\mu$ & $\sigma$ & q1 & q2 & q3\\\hline

		expected lookup time & [ms] &446 & NA & NA & NA & NA\\\hline

		network usage& [MB] & 248 & 13 & 233 & 255 & 257\\\hline

		workload lookup time (sec. ULM)& [ms] & 418 & 198 & 276 & 412 & 543\\\hline

		time until lookup failed (sec. ULM)& [ms] & 411 & 6669 & 177 & 184 & 231\\\hline

		workload error rate (sec. ULM)& [\%] & 6 & 1 & 5 & 6 & 6\\\hline

		\end{tabular}

		\caption{{\footnotesize ULM distributions, measured with managed nodes (policy 1). 

}}

		\begin{tabular}[t]{|l|r|r|r|r|r|r|}

		\hline user-level metric & unit &  $\mu$ & $\sigma$ & q1 & q2 & q3\\\hline

		expected lookup time & [ms] &515 & NA & NA & NA & NA\\\hline

		network usage& [MB] & 211 & 22 & 191 & 208 & 234\\\hline

		workload lookup time (sec. ULM)& [ms] & 444 & 185 & 304 & 425 & 560\\\hline

		time until lookup failed (sec. ULM)& [ms] & 916 & 12514 & 179 & 185 & 233\\\hline

		workload error rate (sec. ULM)& [\%] & 7 & 1 & 6 & 7 & 8\\\hline

		\end{tabular}

		\caption{{\footnotesize ULM distributions, measured with managed nodes (policy 2). 

}}

	}

	\end{center}

\end{table}

\newpage

\subsection{\label{sec:WL3_NB1}Synthetic Varied Weight Workload Network with Low Membership Churn}

\begin{figure}[htpb]

	\centerline{{\footnotesize \resizebox{70mm}{!}{\includegraphics{./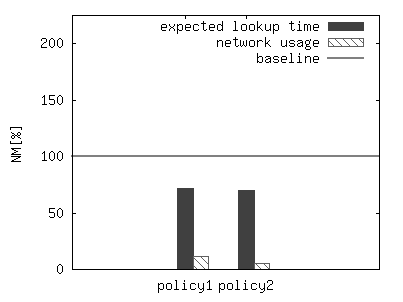}}}}

	\caption{\label{fig:Holistic Synthetic Varied Weight Workload Network with Low Membership Churn user-level metrics} mean normalised monitored ULMs averaged over 3 repetitions (NM)}

\end{figure}

\begin{table}[htpb]

	\begin{center}

	{\footnotesize

		\begin{tabular}[t]{|l|r|r|r|r|r|r|}

		\hline user-level metric & unit &  $\mu$ & $\sigma$ & q1 & q2 & q3\\\hline

		expected lookup time & [ms] &638 & NA & NA & NA & NA\\\hline

		network usage& [MB] & 752 & 4 & 748 & 754 & 755\\\hline

		workload lookup time (sec. ULM)& [ms] & 638 & 235 & 461 & 643 & 797\\\hline

		workload error rate (sec. ULM) & [\%] & 0 & 0 & 0 & 0 & 0 \\\hline

		\end{tabular}

		\caption{{\footnotesize ULM distributions, measured with unmanaged nodes. 

}}

		\begin{tabular}[t]{|l|r|r|r|r|r|r|}

		\hline user-level metric & unit &  $\mu$ & $\sigma$ & q1 & q2 & q3\\\hline

		expected lookup time & [ms] &454 & NA & NA & NA & NA\\\hline

		network usage& [MB] & 77 & 0 & 77 & 77 & 77\\\hline

		workload lookup time (sec. ULM)& [ms] & 454 & 152 & 366 & 455 & 565\\\hline

		workload error rate (sec. ULM) & [\%] & 0 & 0 & 0 & 0 & 0 \\\hline

		\end{tabular}

		\caption{{\footnotesize ULM distributions, measured with managed nodes (policy 1). 

}}

		\begin{tabular}[t]{|l|r|r|r|r|r|r|}

		\hline user-level metric & unit &  $\mu$ & $\sigma$ & q1 & q2 & q3\\\hline

		expected lookup time & [ms] &445 & NA & NA & NA & NA\\\hline

		network usage& [MB] & 37 & 0 & 37 & 37 & 37\\\hline

		workload lookup time (sec. ULM)& [ms] & 445 & 142 & 363 & 452 & 554\\\hline

		workload error rate (sec. ULM) & [\%] & 0 & 0 & 0 & 0 & 0 \\\hline

		\end{tabular}

		\caption{{\footnotesize ULM distributions, measured with managed nodes (policy 2). 

}}

	}

	\end{center}

\end{table}

\newpage

\subsection{\label{sec:WL3_NB2}Synthetic Varied Weight Workload Network with High Membership Churn}

\begin{figure}[htpb]

	\centerline{{\footnotesize \resizebox{70mm}{!}{\includegraphics{./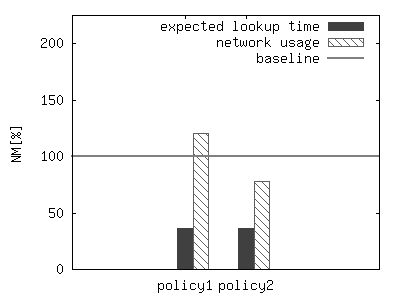}}}}

	\caption{\label{fig:Holistic Synthetic Varied Weight Workload Network with High Membership Churn user-level metrics} mean normalised monitored ULMs averaged over 3 repetitions (NM)}

\end{figure}

\begin{table}[htpb]

	\begin{center}

	{\footnotesize

		\begin{tabular}[t]{|l|r|r|r|r|r|r|}

		\hline user-level metric & unit &  $\mu$ & $\sigma$ & q1 & q2 & q3\\\hline

		expected lookup time & [ms] &1089 & NA & NA & NA & NA\\\hline

		network usage& [MB] & 183 & 207 & 11 & 125 & 413\\\hline

		workload lookup time (sec. ULM)& [ms] & 566 & 277 & 373 & 555 & 722\\\hline

		time until lookup failed (sec. ULM)& [ms] & 243 & 3572 & 97 & 102 & 107\\\hline

		workload error rate (sec. ULM)& [\%] & 50 & 42 & 4 & 60 & 86\\\hline

		\end{tabular}

		\caption{{\footnotesize ULM distributions, measured with unmanaged nodes. 

}}

		\begin{tabular}[t]{|l|r|r|r|r|r|r|}

		\hline user-level metric & unit &  $\mu$ & $\sigma$ & q1 & q2 & q3\\\hline

		expected lookup time & [ms] &423 & NA & NA & NA & NA\\\hline

		network usage& [MB] & 227 & 8 & 218 & 231 & 232\\\hline

		workload lookup time (sec. ULM)& [ms] & 405 & 194 & 274 & 371 & 519\\\hline

		time until lookup failed (sec. ULM)& [ms] & 122 & 105 & 85 & 87 & 144\\\hline

		workload error rate (sec. ULM)& [\%] & 10 & 5 & 4 & 12 & 13\\\hline

		\end{tabular}

		\caption{{\footnotesize ULM distributions, measured with managed nodes (policy 1). 

}}

		\begin{tabular}[t]{|l|r|r|r|r|r|r|}

		\hline user-level metric & unit &  $\mu$ & $\sigma$ & q1 & q2 & q3\\\hline

		expected lookup time & [ms] &423 & NA & NA & NA & NA\\\hline

		network usage& [MB] & 147 & 19 & 130 & 144 & 168\\\hline

		workload lookup time (sec. ULM)& [ms] & 389 & 202 & 244 & 354 & 506\\\hline

		time until lookup failed (sec. ULM)& [ms] & 174 & 106 & 86 & 183 & 233\\\hline

		workload error rate (sec. ULM)& [\%] & 13 & 3 & 10 & 15 & 16\\\hline

		\end{tabular}

		\caption{{\footnotesize ULM distributions, measured with managed nodes (policy 2). 

}}

	}

	\end{center}

\end{table}

\newpage

\subsection{\label{sec:WL3_NB3}Synthetic Varied Weight Workload Network with Locally Varying Membership Churn}

\begin{figure}[htpb]

	\centerline{{\footnotesize \resizebox{70mm}{!}{\includegraphics{./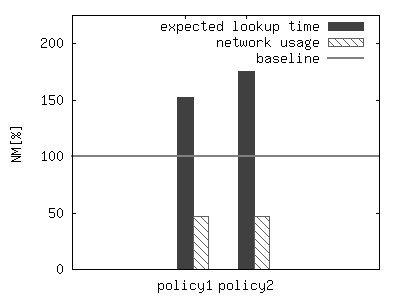}}}}

	\caption{\label{fig:Holistic Synthetic Varied Weight Workload Network with Locally Varying Membership Churn user-level metrics} mean normalised monitored ULMs averaged over 3 repetitions (NM)}

\end{figure}

\begin{table}[htpb]

	\begin{center}

	{\footnotesize

		\begin{tabular}[t]{|l|r|r|r|r|r|r|}

		\hline user-level metric & unit &  $\mu$ & $\sigma$ & q1 & q2 & q3\\\hline

		expected lookup time & [ms] &580 & NA & NA & NA & NA\\\hline

		network usage& [MB] & 496 & 3 & 492 & 498 & 499\\\hline

		workload lookup time (sec. ULM)& [ms] & 570 & 267 & 367 & 551 & 758\\\hline

		time until lookup failed (sec. ULM)& [ms] & 966 & 1021 & 195 & 389 & 1726\\\hline

		workload error rate (sec. ULM)& [\%] & 1 & 1 & 1 & 1 & 2\\\hline

		\end{tabular}

		\caption{{\footnotesize ULM distributions, measured with unmanaged nodes. 

}}

		\begin{tabular}[t]{|l|r|r|r|r|r|r|}

		\hline user-level metric & unit &  $\mu$ & $\sigma$ & q1 & q2 & q3\\\hline

		expected lookup time & [ms] &880 & NA & NA & NA & NA\\\hline

		network usage& [MB] & 231 & 9 & 225 & 227 & 242\\\hline

		workload lookup time (sec. ULM)& [ms] & 444 & 200 & 282 & 427 & 589\\\hline

		time until lookup failed (sec. ULM)& [ms] & 6804 & 34634 & 143 & 188 & 279\\\hline

		workload error rate (sec. ULM)& [\%] & 6 & 0 & 5 & 6 & 6\\\hline

		\end{tabular}

		\caption{{\footnotesize ULM distributions, measured with managed nodes (policy 1). 

}}

		\begin{tabular}[t]{|l|r|r|r|r|r|r|}

		\hline user-level metric & unit &  $\mu$ & $\sigma$ & q1 & q2 & q3\\\hline

		expected lookup time & [ms] &1013 & NA & NA & NA & NA\\\hline

		network usage& [MB] & 234 & 57 & 175 & 239 & 289\\\hline

		workload lookup time (sec. ULM)& [ms] & 572 & 477 & 279 & 470 & 673\\\hline

		time until lookup failed (sec. ULM)& [ms] & 2413 & 18462 & 52 & 183 & 239\\\hline

		workload error rate (sec. ULM)& [\%] & 15 & 8 & 7 & 14 & 24\\\hline

		\end{tabular}

		\caption{{\footnotesize ULM distributions, measured with managed nodes (policy 2). 

}}

	}

	\end{center}

\end{table}

\newpage

\subsection{\label{sec:WL3_NB4}Synthetic Varied Weight Workload Network with Temporal Varying Membership Churn}

\begin{figure}[htpb]

	\centerline{{\footnotesize \resizebox{70mm}{!}{\includegraphics{./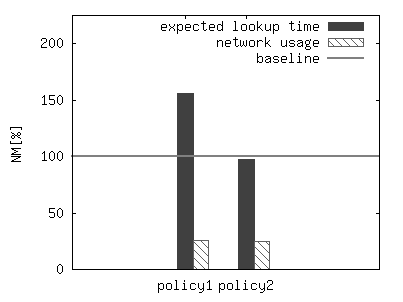}}}}

	\caption{\label{fig:Holistic Synthetic Varied Weight Workload Network with Temporal Varying Membership Churn user-level metrics} mean normalised monitored ULMs averaged over 3 repetitions (NM)}

\end{figure}

\begin{table}[htpb]

	\begin{center}

	{\footnotesize

		\begin{tabular}[t]{|l|r|r|r|r|r|r|}

		\hline user-level metric & unit &  $\mu$ & $\sigma$ & q1 & q2 & q3\\\hline

		expected lookup time & [ms] &577 & NA & NA & NA & NA\\\hline

		network usage& [MB] & 575 & 3 & 572 & 575 & 577\\\hline

		workload lookup time (sec. ULM)& [ms] & 575 & 257 & 390 & 552 & 735\\\hline

		time until lookup failed (sec. ULM)& [ms] & 162 & 144 & 49 & 143 & 231\\\hline

		workload error rate (sec. ULM)& [\%] & 1 & 0 & 1 & 1 & 1\\\hline

		\end{tabular}

		\caption{{\footnotesize ULM distributions, measured with unmanaged nodes. 

}}

		\begin{tabular}[t]{|l|r|r|r|r|r|r|}

		\hline user-level metric & unit &  $\mu$ & $\sigma$ & q1 & q2 & q3\\\hline

		expected lookup time & [ms] &874 & NA & NA & NA & NA\\\hline

		network usage& [MB] & 166 & 11 & 158 & 161 & 178\\\hline

		workload lookup time (sec. ULM)& [ms] & 435 & 168 & 312 & 418 & 540\\\hline

		time until lookup failed (sec. ULM)& [ms] & 8327 & 103703 & 85 & 86 & 144\\\hline

		workload error rate (sec. ULM)& [\%] & 5 & 6 & 2 & 3 & 12\\\hline

		\end{tabular}

		\caption{{\footnotesize ULM distributions, measured with managed nodes (policy 1). 

}}

		\begin{tabular}[t]{|l|r|r|r|r|r|r|}

		\hline user-level metric & unit &  $\mu$ & $\sigma$ & q1 & q2 & q3\\\hline

		expected lookup time & [ms] &542 & NA & NA & NA & NA\\\hline

		network usage& [MB] & 141 & 36 & 99 & 159 & 164\\\hline

		workload lookup time (sec. ULM)& [ms] & 479 & 186 & 362 & 461 & 588\\\hline

		time until lookup failed (sec. ULM)& [ms] & 252 & 725 & 181 & 224 & 267\\\hline

		workload error rate (sec. ULM)& [\%] & 16 & 4 & 12 & 18 & 20\\\hline

		\end{tabular}

		\caption{{\footnotesize ULM distributions, measured with managed nodes (policy 2). 

}}

	}

	\end{center}

\end{table}

\newpage

\subsection{\label{sec:WL4_NB1}File System Workload Network with Low Membership Churn}

\begin{figure}[htpb]

	\centerline{{\footnotesize \resizebox{70mm}{!}{\includegraphics{./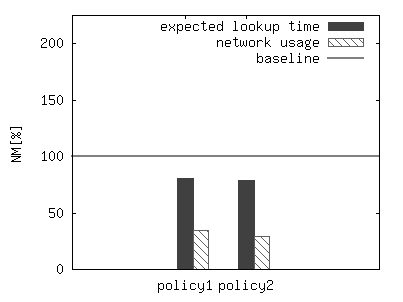}}}}

	\caption{\label{fig:Holistic File System Workload Network with Low Membership Churn user-level metrics} mean normalised monitored ULMs averaged over 3 repetitions (NM)}

\end{figure}

\begin{table}[htpb]

	\begin{center}

	{\footnotesize

		\begin{tabular}[t]{|l|r|r|r|r|r|r|}

		\hline user-level metric & unit &  $\mu$ & $\sigma$ & q1 & q2 & q3\\\hline

		expected lookup time & [ms] &876 & NA & NA & NA & NA\\\hline

		network usage& [MB] & 1400 & 27 & 1377 & 1394 & 1429\\\hline

		workload lookup time (sec. ULM)& [ms] & 876 & 314 & 655 & 899 & 1110\\\hline

		time until lookup failed (sec. ULM)& [ms] & 78 & 0 & 78 & 78 & 78\\\hline

		workload error rate (sec. ULM)& [\%] & 0 & 0 & 0 & 0 & 0\\\hline

		\end{tabular}

		\caption{{\footnotesize ULM distributions, measured with unmanaged nodes. 

}}

		\begin{tabular}[t]{|l|r|r|r|r|r|r|}

		\hline user-level metric & unit &  $\mu$ & $\sigma$ & q1 & q2 & q3\\\hline

		expected lookup time & [ms] &705 & NA & NA & NA & NA\\\hline

		network usage& [MB] & 365 & 0 & 365 & 365 & 365\\\hline

		workload lookup time (sec. ULM)& [ms] & 705 & 244 & 541 & 742 & 899\\\hline

		workload error rate (sec. ULM) & [\%] & 0 & 0 & 0 & 0 & 0 \\\hline

		\end{tabular}

		\caption{{\footnotesize ULM distributions, measured with managed nodes (policy 1). 

}}

		\begin{tabular}[t]{|l|r|r|r|r|r|r|}

		\hline user-level metric & unit &  $\mu$ & $\sigma$ & q1 & q2 & q3\\\hline

		expected lookup time & [ms] &690 & NA & NA & NA & NA\\\hline

		network usage& [MB] & 306 & 0 & 306 & 306 & 306\\\hline

		workload lookup time (sec. ULM)& [ms] & 690 & 238 & 530 & 726 & 887\\\hline

		workload error rate (sec. ULM) & [\%] & 0 & 0 & 0 & 0 & 0 \\\hline

		\end{tabular}

		\caption{{\footnotesize ULM distributions, measured with managed nodes (policy 2). 

}}

	}

	\end{center}

\end{table}

\newpage

\subsection{\label{sec:WL4_NB2}File System Workload Network with High Membership Churn}

\begin{figure}[htpb]

	\centerline{{\footnotesize \resizebox{70mm}{!}{\includegraphics{./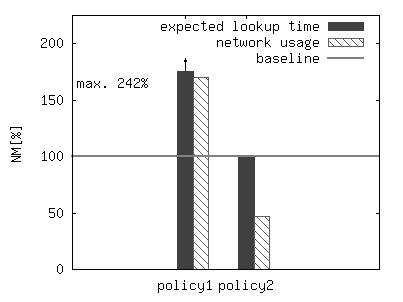}}}}

	\caption{\label{fig:Holistic File System Workload Network with High Membership Churn user-level metrics} mean normalised monitored ULMs averaged over 3 repetitions (NM)}

\end{figure}

\begin{table}[htpb]

	\begin{center}

	{\footnotesize

		\begin{tabular}[t]{|l|r|r|r|r|r|r|}

		\hline user-level metric & unit &  $\mu$ & $\sigma$ & q1 & q2 & q3\\\hline

		expected lookup time & [ms] &838 & NA & NA & NA & NA\\\hline

		network usage& [MB] & 580 & 323 & 207 & 763 & 770\\\hline

		workload lookup time (sec. ULM)& [ms] & 726 & 341 & 506 & 715 & 934\\\hline

		time until lookup failed (sec. ULM)& [ms] & 129 & 341 & 64 & 89 & 126\\\hline

		workload error rate (sec. ULM)& [\%] & 26 & 41 & 3 & 3 & 73\\\hline

		\end{tabular}

		\caption{{\footnotesize ULM distributions, measured with unmanaged nodes. 

}}

		\begin{tabular}[t]{|l|r|r|r|r|r|r|}

		\hline user-level metric & unit &  $\mu$ & $\sigma$ & q1 & q2 & q3\\\hline

		expected lookup time & [ms] &2031 & NA & NA & NA & NA\\\hline

		network usage& [MB] & 985 & 395 & 529 & 1212 & 1215\\\hline

		workload lookup time (sec. ULM)& [ms] & 1497 & 1970 & 506 & 732 & 1092\\\hline

		time until lookup failed (sec. ULM)& [ms] & 3736 & 205918 & 80 & 142 & 375\\\hline

		workload error rate (sec. ULM)& [\%] & 12 & 13 & 4 & 5 & 26\\\hline

		\end{tabular}

		\caption{{\footnotesize ULM distributions, measured with managed nodes (policy 1). 

}}

		\begin{tabular}[t]{|l|r|r|r|r|r|r|}

		\hline user-level metric & unit &  $\mu$ & $\sigma$ & q1 & q2 & q3\\\hline

		expected lookup time & [ms] &834 & NA & NA & NA & NA\\\hline

		network usage& [MB] & 272 & 186 & 57 & 374 & 385\\\hline

		workload lookup time (sec. ULM)& [ms] & 609 & 271 & 418 & 616 & 781\\\hline

		time until lookup failed (sec. ULM)& [ms] & 230 & 3153 & 72 & 118 & 183\\\hline

		workload error rate (sec. ULM)& [\%] & 34 & 41 & 8 & 13 & 81\\\hline

		\end{tabular}

		\caption{{\footnotesize ULM distributions, measured with managed nodes (policy 2). 

}}

	}

	\end{center}

\end{table}

\newpage

\subsection{\label{sec:WL4_NB3}File System Workload Network with Locally Varying Membership Churn}

\begin{figure}[htpb]

	\centerline{{\footnotesize \resizebox{70mm}{!}{\includegraphics{./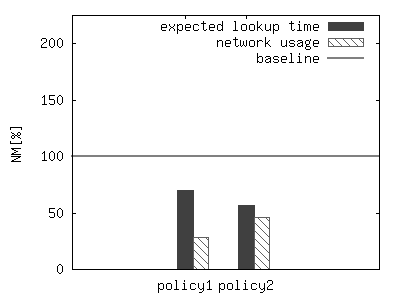}}}}

	\caption{\label{fig:Holistic File System Workload Network with Locally Varying Membership Churn user-level metrics} mean normalised monitored ULMs averaged over 3 repetitions (NM)}

\end{figure}

\begin{table}[htpb]

	\begin{center}

	{\footnotesize

		\begin{tabular}[t]{|l|r|r|r|r|r|r|}

		\hline user-level metric & unit &  $\mu$ & $\sigma$ & q1 & q2 & q3\\\hline

		expected lookup time & [ms] &2366 & NA & NA & NA & NA\\\hline

		network usage& [MB] & 1838 & 659 & 1292 & 1652 & 2571\\\hline

		workload lookup time (sec. ULM)& [ms] & 1821 & 1991 & 591 & 925 & 2479\\\hline

		time until lookup failed (sec. ULM)& [ms] & 6117 & 28939 & 191 & 449 & 993\\\hline

		workload error rate (sec. ULM)& [\%] & 8 & 8 & 3 & 5 & 17\\\hline

		\end{tabular}

		\caption{{\footnotesize ULM distributions, measured with unmanaged nodes. 

}}

		\begin{tabular}[t]{|l|r|r|r|r|r|r|}

		\hline user-level metric & unit &  $\mu$ & $\sigma$ & q1 & q2 & q3\\\hline

		expected lookup time & [ms] &1651 & NA & NA & NA & NA\\\hline

		network usage& [MB] & 519 & 195 & 295 & 613 & 650\\\hline

		workload lookup time (sec. ULM)& [ms] & 1053 & 946 & 529 & 759 & 1051\\\hline

		time until lookup failed (sec. ULM)& [ms] & 2027 & 15234 & 90 & 368 & 852\\\hline

		workload error rate (sec. ULM)& [\%] & 21 & 22 & 8 & 9 & 47\\\hline

		\end{tabular}

		\caption{{\footnotesize ULM distributions, measured with managed nodes (policy 1). 

}}

		\begin{tabular}[t]{|l|r|r|r|r|r|r|}

		\hline user-level metric & unit &  $\mu$ & $\sigma$ & q1 & q2 & q3\\\hline

		expected lookup time & [ms] &1340 & NA & NA & NA & NA\\\hline

		network usage& [MB] & 854 & 285 & 672 & 708 & 1183\\\hline

		workload lookup time (sec. ULM)& [ms] & 798 & 571 & 453 & 709 & 943\\\hline

		time until lookup failed (sec. ULM)& [ms] & 2716 & 21396 & 99 & 360 & 562\\\hline

		workload error rate (sec. ULM)& [\%] & 16 & 11 & 7 & 12 & 29\\\hline

		\end{tabular}

		\caption{{\footnotesize ULM distributions, measured with managed nodes (policy 2). 

}}

	}

	\end{center}

\end{table}

\newpage

\subsection{\label{sec:WL4_NB4}File System Workload Network with Temporal Varying Membership Churn}

\begin{figure}[htpb]

	\centerline{{\footnotesize \resizebox{70mm}{!}{\includegraphics{./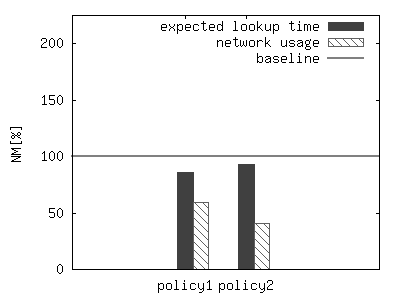}}}}

	\caption{\label{fig:Holistic File System Workload Network with Temporal Varying Membership Churn user-level metrics} mean normalised monitored ULMs averaged over 3 repetitions (NM)}

\end{figure}

\begin{table}[htpb]

	\begin{center}

	{\footnotesize

		\begin{tabular}[t]{|l|r|r|r|r|r|r|}

		\hline user-level metric & unit &  $\mu$ & $\sigma$ & q1 & q2 & q3\\\hline

		expected lookup time & [ms] &785 & NA & NA & NA & NA\\\hline

		network usage& [MB] & 904 & 157 & 723 & 979 & 1009\\\hline

		workload lookup time (sec. ULM)& [ms] & 770 & 322 & 551 & 783 & 1004\\\hline

		time until lookup failed (sec. ULM)& [ms] & 114 & 232 & 47 & 54 & 73\\\hline

		workload error rate (sec. ULM)& [\%] & 8 & 11 & 1 & 1 & 21\\\hline

		\end{tabular}

		\caption{{\footnotesize ULM distributions, measured with unmanaged nodes. 

}}

		\begin{tabular}[t]{|l|r|r|r|r|r|r|}

		\hline user-level metric & unit &  $\mu$ & $\sigma$ & q1 & q2 & q3\\\hline

		expected lookup time & [ms] &673 & NA & NA & NA & NA\\\hline

		network usage& [MB] & 458 & 21 & 435 & 459 & 478\\\hline

		workload lookup time (sec. ULM)& [ms] & 654 & 263 & 471 & 669 & 842\\\hline

		time until lookup failed (sec. ULM)& [ms] & 330 & 258 & 211 & 327 & 414\\\hline

		workload error rate (sec. ULM)& [\%] & 5 & 1 & 4 & 5 & 6\\\hline

		\end{tabular}

		\caption{{\footnotesize ULM distributions, measured with managed nodes (policy 1). 

}}

		\begin{tabular}[t]{|l|r|r|r|r|r|r|}

		\hline user-level metric & unit &  $\mu$ & $\sigma$ & q1 & q2 & q3\\\hline

		expected lookup time & [ms] &713 & NA & NA & NA & NA\\\hline

		network usage& [MB] & 361 & 46 & 328 & 342 & 414\\\hline

		workload lookup time (sec. ULM)& [ms] & 608 & 273 & 388 & 617 & 817\\\hline

		time until lookup failed (sec. ULM)& [ms] & 1002 & 25285 & 145 & 282 & 381\\\hline

		workload error rate (sec. ULM)& [\%] & 9 & 4 & 6 & 7 & 13\\\hline

		\end{tabular}

		\caption{{\footnotesize ULM distributions, measured with managed nodes (policy 2). 

}}

	}

	\end{center}

\end{table}
