# Supplementary material for: Autonomic Management in a Distributed Storage System
Source: arXiv:1007.0328 source file (2010-07-02)
Supplement: Supplementary file 3 [file p2p_main_results.tex]

\subsection{\label{sec:WL1_NB1}Syn. Light Weight Workload and Low Churn}

\begin{figure}[h!tpb]
	\centerline{{\footnotesize \resizebox{70mm}{!}{\includegraphics{./appendix/reportFigures/averaged_user-level_metrics.png}}}}
	\caption{\label{fig:Synthetic Light Weight Workload and Low Membership Churn user-level metrics} mean normalised monitored ULMs averaged over 3 repetitions (NM)}
\end{figure}
\begin{table}[h!tpb]
	\begin{center}
	{\footnotesize
		\begin{tabular}[t]{|l|r|r|r|r|r|}
		\hline user-level metric & unit &  mean & std & median & $1^{st}$ quartile \\\hline
		expected lookup time & [ms] &720 & NA & NA & NA  \\\hline
		network usage& [MB] & 599 & 8 & 603 & 590\\\hline
		workload lookup time (sec. ULM)& [ms] & 720 & 207 & 777 & 516\\\hline
		workload error rate (sec. ULM) & [\%] & 0 & 0 & 0 & 0 \\\hline
		\end{tabular}

		\caption{{\footnotesize Raw ULMs averaged over 3 repetitions in a network with unmanaged nodes. 
}}
		\begin{tabular}[t]{|l|r|r|r|r|r|}
		\hline user-level metric & unit &  mean & std & median & $1^{st}$ quartile \\\hline
		expected lookup time & [ms] &522 & NA & NA & NA  \\\hline
		network usage& [MB] & 54 & 0 & 54 & 54\\\hline
		workload lookup time (sec. ULM)& [ms] & 522 & 145 & 535 & 406\\\hline
		workload error rate (sec. ULM) & [\%] & 0 & 0 & 0 & 0 \\\hline
		\end{tabular}

		\caption{{\footnotesize Raw ULMs averaged over 3 repetitions in a network with managed nodes (policy 1). 
}}
		\begin{tabular}[t]{|l|r|r|r|r|r|}
		\hline user-level metric & unit &  mean & std & median & $1^{st}$ quartile \\\hline
		expected lookup time & [ms] &507 & NA & NA & NA  \\\hline
		network usage& [MB] & 17 & 0 & 17 & 17\\\hline
		workload lookup time (sec. ULM)& [ms] & 507 & 121 & 567 & 425\\\hline
		workload error rate (sec. ULM) & [\%] & 0 & 0 & 0 & 0 \\\hline
		\end{tabular}

		\caption{{\footnotesize Raw ULMs averaged over 3 repetitions in a network with managed nodes (policy 2). 
}}
	}
	\end{center}
\end{table}
\newpage
\subsection{\label{sec:WL1_NB2}Syn. Light Weight Workload and High Churn}

\begin{figure}[h!tpb]
	\centerline{{\footnotesize \resizebox{70mm}{!}{\includegraphics{./appendix/reportFigures/averaged_user-level_metrics.png}}}}
	\caption{\label{fig:Synthetic Light Weight Workload and High Membership Churn user-level metrics} mean normalised monitored ULMs averaged over 3 repetitions (NM)}
\end{figure}
\begin{table}[h!tpb]
	\begin{center}
	{\footnotesize
		\begin{tabular}[t]{|l|r|r|r|r|r|}
		\hline user-level metric & unit &  mean & std & median & $1^{st}$ quartile \\\hline
		expected lookup time & [ms] &566 & NA & NA & NA  \\\hline
		network usage& [MB] & 327 & 28 & 333 & 296\\\hline
		workload lookup time (sec. ULM)& [ms] & 562 & 296 & 551 & 398\\\hline
		time until lookup failed (sec. ULM)& [ms] & 11 & 4 & 11 & 8\\\hline
		workload error rate (sec. ULM)& [\%] & 7 & 12 & 0 & 0\\\hline
		\end{tabular}

		\caption{{\footnotesize Raw ULMs averaged over 3 repetitions in a network with unmanaged nodes. 
}}
		\begin{tabular}[t]{|l|r|r|r|r|r|}
		\hline user-level metric & unit &  mean & std & median & $1^{st}$ quartile \\\hline
		expected lookup time & [ms] &7584 & NA & NA & NA  \\\hline
		network usage& [MB] & 179 & 11 & 183 & 167\\\hline
		workload lookup time (sec. ULM)& [ms] & 457 & 166 & 482 & 386\\\hline
		time until lookup failed (sec. ULM)& [ms] & 16493 & 49431 & 17 & 13\\\hline
		workload error rate (sec. ULM)& [\%] & 30 & 10 & 30 & 20\\\hline
		\end{tabular}

		\caption{{\footnotesize Raw ULMs averaged over 3 repetitions in a network with managed nodes (policy 1). 
}}
		\begin{tabular}[t]{|l|r|r|r|r|r|}
		\hline user-level metric & unit &  mean & std & median & $1^{st}$ quartile \\\hline
		expected lookup time & [ms] &7930 & NA & NA & NA  \\\hline
		network usage& [MB] & 116 & 5 & 113 & 113\\\hline
		workload lookup time (sec. ULM)& [ms] & 459 & 265 & 428 & 311\\\hline
		time until lookup failed (sec. ULM)& [ms] & 12555 & 41412 & 47 & 13\\\hline
		workload error rate (sec. ULM)& [\%] & 37 & 12 & 30 & 30\\\hline
		\end{tabular}

		\caption{{\footnotesize Raw ULMs averaged over 3 repetitions in a network with managed nodes (policy 2). 
}}
	}
	\end{center}
\end{table}
\newpage
\subsection{\label{sec:WL1_NB3}Syn. Light Weight Workload and Locally Varying Churn}

\begin{figure}[h!tpb]
	\centerline{{\footnotesize \resizebox{70mm}{!}{\includegraphics{./appendix/reportFigures/averaged_user-level_metrics.png}}}}
	\caption{\label{fig:Synthetic Light Weight Workload and Locally Varying Membership Churn user-level metrics} mean normalised monitored ULMs averaged over 3 repetitions (NM)}
\end{figure}
\begin{table}[h!tpb]
	\begin{center}
	{\footnotesize
		\begin{tabular}[t]{|l|r|r|r|r|r|}
		\hline user-level metric & unit &  mean & std & median & $1^{st}$ quartile \\\hline
		expected lookup time & [ms] &689 & NA & NA & NA  \\\hline
		network usage& [MB] & 396 & 8 & 399 & 387\\\hline
		workload lookup time (sec. ULM)& [ms] & 689 & 248 & 708 & 550\\\hline
		workload error rate (sec. ULM) & [\%] & 0 & 0 & 0 & 0 \\\hline
		\end{tabular}

		\caption{{\footnotesize Raw ULMs averaged over 3 repetitions in a network with unmanaged nodes. 
}}
		\begin{tabular}[t]{|l|r|r|r|r|r|}
		\hline user-level metric & unit &  mean & std & median & $1^{st}$ quartile \\\hline
		expected lookup time & [ms] &614 & NA & NA & NA  \\\hline
		network usage& [MB] & 180 & 1 & 179 & 179\\\hline
		workload lookup time (sec. ULM)& [ms] & 575 & 224 & 612 & 422\\\hline
		time until lookup failed (sec. ULM)& [ms] & 186 & 133 & 201 & 55\\\hline
		workload error rate (sec. ULM)& [\%] & 13 & 6 & 10 & 10\\\hline
		\end{tabular}

		\caption{{\footnotesize Raw ULMs averaged over 3 repetitions in a network with managed nodes (policy 1). 
}}
		\begin{tabular}[t]{|l|r|r|r|r|r|}
		\hline user-level metric & unit &  mean & std & median & $1^{st}$ quartile \\\hline
		expected lookup time & [ms] &856 & NA & NA & NA  \\\hline
		network usage& [MB] & 173 & 37 & 187 & 132\\\hline
		workload lookup time (sec. ULM)& [ms] & 831 & 574 & 701 & 448\\\hline
		time until lookup failed (sec. ULM)& [ms] & 56 & 93 & 11 & 9\\\hline
		workload error rate (sec. ULM)& [\%] & 13 & 6 & 10 & 10\\\hline
		\end{tabular}

		\caption{{\footnotesize Raw ULMs averaged over 3 repetitions in a network with managed nodes (policy 2). 
}}
	}
	\end{center}
\end{table}
\newpage
\subsection{\label{sec:WL1_NB4}Syn. Light Weight Workload and Locally Varying Churn}

\begin{figure}[h!tpb]
	\centerline{{\footnotesize \resizebox{70mm}{!}{\includegraphics{./appendix/reportFigures/averaged_user-level_metrics.png}}}}
	\caption{\label{fig:Synthetic Light Weight Workload and Locally Varying Membership Churn user-level metrics} mean normalised monitored ULMs averaged over 3 repetitions (NM)}
\end{figure}
\begin{table}[h!tpb]
	\begin{center}
	{\footnotesize
		\begin{tabular}[t]{|l|r|r|r|r|r|}
		\hline user-level metric & unit &  mean & std & median & $1^{st}$ quartile \\\hline
		expected lookup time & [ms] &715 & NA & NA & NA  \\\hline
		network usage& [MB] & 437 & 26 & 446 & 408\\\hline
		workload lookup time (sec. ULM)& [ms] & 643 & 232 & 602 & 463\\\hline
		time until lookup failed (sec. ULM)& [ms] & 397 & 767 & 14 & 13\\\hline
		workload error rate (sec. ULM)& [\%] & 13 & 6 & 10 & 10\\\hline
		\end{tabular}

		\caption{{\footnotesize Raw ULMs averaged over 3 repetitions in a network with unmanaged nodes. 
}}
		\begin{tabular}[t]{|l|r|r|r|r|r|}
		\hline user-level metric & unit &  mean & std & median & $1^{st}$ quartile \\\hline
		expected lookup time & [ms] &525 & NA & NA & NA  \\\hline
		network usage& [MB] & 128 & 15 & 124 & 116\\\hline
		workload lookup time (sec. ULM)& [ms] & 518 & 152 & 466 & 441\\\hline
		time until lookup failed (sec. ULM)& [ms] & 12 & 0 & 12 & 12\\\hline
		workload error rate (sec. ULM)& [\%] & 10 & 0 & 10 & 10\\\hline
		\end{tabular}

		\caption{{\footnotesize Raw ULMs averaged over 3 repetitions in a network with managed nodes (policy 1). 
}}
		\begin{tabular}[t]{|l|r|r|r|r|r|}
		\hline user-level metric & unit &  mean & std & median & $1^{st}$ quartile \\\hline
		expected lookup time & [ms] &3010 & NA & NA & NA  \\\hline
		network usage& [MB] & 78 & 25 & 67 & 61\\\hline
		workload lookup time (sec. ULM)& [ms] & 629 & 503 & 466 & 311\\\hline
		time until lookup failed (sec. ULM)& [ms] & 15855 & 18374 & 14820 & 9\\\hline
		workload error rate (sec. ULM)& [\%] & 13 & 6 & 10 & 10\\\hline
		\end{tabular}

		\caption{{\footnotesize Raw ULMs averaged over 3 repetitions in a network with managed nodes (policy 2). 
}}
	}
	\end{center}
\end{table}
\newpage
\subsection{\label{sec:WL2_NB1}Syn. Heavy Weight Workload and Low Churn}

\begin{figure}[h!tpb]
	\centerline{{\footnotesize \resizebox{70mm}{!}{\includegraphics{./appendix/reportFigures/averaged_user-level_metrics.png}}}}
	\caption{\label{fig:Synthetic Heavy Weight Workload and Low Membership Churn user-level metrics} mean normalised monitored ULMs averaged over 3 repetitions (NM)}
\end{figure}
\begin{table}[h!tpb]
	\begin{center}
	{\footnotesize
		\begin{tabular}[t]{|l|r|r|r|r|r|}
		\hline user-level metric & unit &  mean & std & median & $1^{st}$ quartile \\\hline
		expected lookup time & [ms] &613 & NA & NA & NA  \\\hline
		network usage& [MB] & 891 & 1 & 891 & 890\\\hline
		workload lookup time (sec. ULM)& [ms] & 613 & 228 & 615 & 444\\\hline
		workload error rate (sec. ULM) & [\%] & 0 & 0 & 0 & 0 \\\hline
		\end{tabular}

		\caption{{\footnotesize Raw ULMs averaged over 3 repetitions in a network with unmanaged nodes. 
}}
		\begin{tabular}[t]{|l|r|r|r|r|r|}
		\hline user-level metric & unit &  mean & std & median & $1^{st}$ quartile \\\hline
		expected lookup time & [ms] &445 & NA & NA & NA  \\\hline
		network usage& [MB] & 194 & 1 & 194 & 193\\\hline
		workload lookup time (sec. ULM)& [ms] & 445 & 152 & 445 & 354\\\hline
		workload error rate (sec. ULM) & [\%] & 0 & 0 & 0 & 0 \\\hline
		\end{tabular}

		\caption{{\footnotesize Raw ULMs averaged over 3 repetitions in a network with managed nodes (policy 1). 
}}
		\begin{tabular}[t]{|l|r|r|r|r|r|}
		\hline user-level metric & unit &  mean & std & median & $1^{st}$ quartile \\\hline
		expected lookup time & [ms] &428 & NA & NA & NA  \\\hline
		network usage& [MB] & 142 & 1 & 141 & 141\\\hline
		workload lookup time (sec. ULM)& [ms] & 428 & 142 & 419 & 322\\\hline
		time until lookup failed (sec. ULM)& [ms] & 206 & 0 & 206 & 206\\\hline
		workload error rate (sec. ULM)& [\%] & 0 & 0 & 0 & 0\\\hline
		\end{tabular}

		\caption{{\footnotesize Raw ULMs averaged over 3 repetitions in a network with managed nodes (policy 2). 
}}
	}
	\end{center}
\end{table}
\newpage

\subsection{\label{sec:WL2_NB2}Syn. Heavy Weight Workload and High Churn}

\begin{figure}[h!tpb]
	\centerline{{\footnotesize \resizebox{70mm}{!}{\includegraphics{./appendix/reportFigures/averaged_user-level_metrics.png}}}}
	\caption{\label{fig:Synthetic Heavy Weight Workload and High Membership Churn user-level metrics} mean normalised monitored ULMs averaged over 3 repetitions (NM)}
\end{figure}
\begin{table}[h!tpb]
	\begin{center}
	{\footnotesize
		\begin{tabular}[t]{|l|r|r|r|r|r|}
		\hline user-level metric & unit &  mean & std & median & $1^{st}$ quartile \\\hline
		expected lookup time & [ms] &772 & NA & NA & NA  \\\hline
		network usage& [MB] & 230 & 199 & 121 & 109\\\hline
		workload lookup time (sec. ULM)& [ms] & 590 & 256 & 623 & 406\\\hline
		time until lookup failed (sec. ULM)& [ms] & 152 & 1181 & 99 & 67\\\hline
		workload error rate (sec. ULM)& [\%] & 34 & 34 & 29 & 3\\\hline
		\end{tabular}

		\caption{{\footnotesize Raw ULMs averaged over 3 repetitions in a network with unmanaged nodes. 
}}
		\begin{tabular}[t]{|l|r|r|r|r|r|}
		\hline user-level metric & unit &  mean & std & median & $1^{st}$ quartile \\\hline
		expected lookup time & [ms] &443 & NA & NA & NA  \\\hline
		network usage& [MB] & 296 & 3 & 295 & 293\\\hline
		workload lookup time (sec. ULM)& [ms] & 434 & 208 & 412 & 278\\\hline
		time until lookup failed (sec. ULM)& [ms] & 196 & 160 & 185 & 86\\\hline
		workload error rate (sec. ULM)& [\%] & 4 & 0 & 4 & 4\\\hline
		\end{tabular}

		\caption{{\footnotesize Raw ULMs averaged over 3 repetitions in a network with managed nodes (policy 1). 
}}
		\begin{tabular}[t]{|l|r|r|r|r|r|}
		\hline user-level metric & unit &  mean & std & median & $1^{st}$ quartile \\\hline
		expected lookup time & [ms] &474 & NA & NA & NA  \\\hline
		network usage& [MB] & 218 & 21 & 209 & 203\\\hline
		workload lookup time (sec. ULM)& [ms] & 409 & 198 & 389 & 275\\\hline
		time until lookup failed (sec. ULM)& [ms] & 482 & 6545 & 185 & 142\\\hline
		workload error rate (sec. ULM)& [\%] & 11 & 4 & 9 & 8\\\hline
		\end{tabular}

		\caption{{\footnotesize Raw ULMs averaged over 3 repetitions in a network with managed nodes (policy 2). 
}}
	}
	\end{center}
\end{table}
\newpage

\subsection{\label{sec:WL2_NB3}Syn. Heavy Weight Workload and Locally Varying Churn}

\begin{figure}[h!tpb]
	\centerline{{\footnotesize \resizebox{70mm}{!}{\includegraphics{./appendix/reportFigures/averaged_user-level_metrics.png}}}}
	\caption{\label{fig:Synthetic Heavy Weight Workload and Locally Varying Membership Churn user-level metrics} mean normalised monitored ULMs averaged over 3 repetitions (NM)}
\end{figure}
\begin{table}[h!tpb]
	\begin{center}
	{\footnotesize
		\begin{tabular}[t]{|l|r|r|r|r|r|}
		\hline user-level metric & unit &  mean & std & median & $1^{st}$ quartile \\\hline
		expected lookup time & [ms] &1370 & NA & NA & NA  \\\hline
		network usage& [MB] & 529 & 101 & 587 & 412\\\hline
		workload lookup time (sec. ULM)& [ms] & 840 & 657 & 647 & 416\\\hline
		time until lookup failed (sec. ULM)& [ms] & 2447 & 17738 & 166 & 74\\\hline
		workload error rate (sec. ULM)& [\%] & 17 & 14 & 19 & 1\\\hline
		\end{tabular}

		\caption{{\footnotesize Raw ULMs averaged over 3 repetitions in a network with unmanaged nodes. 
}}
		\begin{tabular}[t]{|l|r|r|r|r|r|}
		\hline user-level metric & unit &  mean & std & median & $1^{st}$ quartile \\\hline
		expected lookup time & [ms] &491 & NA & NA & NA  \\\hline
		network usage& [MB] & 296 & 9 & 294 & 288\\\hline
		workload lookup time (sec. ULM)& [ms] & 444 & 204 & 421 & 279\\\hline
		time until lookup failed (sec. ULM)& [ms] & 871 & 12153 & 186 & 143\\\hline
		workload error rate (sec. ULM)& [\%] & 5 & 1 & 5 & 5\\\hline
		\end{tabular}

		\caption{{\footnotesize Raw ULMs averaged over 3 repetitions in a network with managed nodes (policy 1). 
}}
		\begin{tabular}[t]{|l|r|r|r|r|r|}
		\hline user-level metric & unit &  mean & std & median & $1^{st}$ quartile \\\hline
		expected lookup time & [ms] &825 & NA & NA & NA  \\\hline
		network usage& [MB] & 353 & 66 & 322 & 309\\\hline
		workload lookup time (sec. ULM)& [ms] & 541 & 438 & 444 & 283\\\hline
		time until lookup failed (sec. ULM)& [ms] & 1527 & 15181 & 186 & 141\\\hline
		workload error rate (sec. ULM)& [\%] & 16 & 9 & 11 & 10\\\hline
		\end{tabular}

		\caption{{\footnotesize Raw ULMs averaged over 3 repetitions in a network with managed nodes (policy 2). 
}}
	}
	\end{center}
\end{table}
\newpage

\subsection{\label{sec:WL2_NB4}Syn. Heavy Weight Workload and Locally Varying Churn}

\begin{figure}[h!tpb]
	\centerline{{\footnotesize \resizebox{70mm}{!}{\includegraphics{./appendix/reportFigures/averaged_user-level_metrics.png}}}}
	\caption{\label{fig:Synthetic Heavy Weight Workload and Locally Varying Membership Churn user-level metrics} mean normalised monitored ULMs averaged over 3 repetitions (NM)}
\end{figure}
\begin{table}[h!tpb]
	\begin{center}
	{\footnotesize
		\begin{tabular}[t]{|l|r|r|r|r|r|}
		\hline user-level metric & unit &  mean & std & median & $1^{st}$ quartile \\\hline
		expected lookup time & [ms] &655 & NA & NA & NA  \\\hline
		network usage& [MB] & 629 & 84 & 676 & 532\\\hline
		workload lookup time (sec. ULM)& [ms] & 622 & 408 & 570 & 409\\\hline
		time until lookup failed (sec. ULM)& [ms] & 196 & 745 & 105 & 97\\\hline
		workload error rate (sec. ULM)& [\%] & 11 & 17 & 1 & 1\\\hline
		\end{tabular}

		\caption{{\footnotesize Raw ULMs averaged over 3 repetitions in a network with unmanaged nodes. 
}}
		\begin{tabular}[t]{|l|r|r|r|r|r|}
		\hline user-level metric & unit &  mean & std & median & $1^{st}$ quartile \\\hline
		expected lookup time & [ms] &446 & NA & NA & NA  \\\hline
		network usage& [MB] & 248 & 13 & 255 & 233\\\hline
		workload lookup time (sec. ULM)& [ms] & 418 & 198 & 412 & 276\\\hline
		time until lookup failed (sec. ULM)& [ms] & 411 & 6669 & 184 & 177\\\hline
		workload error rate (sec. ULM)& [\%] & 6 & 1 & 6 & 5\\\hline
		\end{tabular}

		\caption{{\footnotesize Raw ULMs averaged over 3 repetitions in a network with managed nodes (policy 1). 
}}
		\begin{tabular}[t]{|l|r|r|r|r|r|}
		\hline user-level metric & unit &  mean & std & median & $1^{st}$ quartile \\\hline
		expected lookup time & [ms] &515 & NA & NA & NA  \\\hline
		network usage& [MB] & 211 & 22 & 208 & 191\\\hline
		workload lookup time (sec. ULM)& [ms] & 444 & 185 & 425 & 304\\\hline
		time until lookup failed (sec. ULM)& [ms] & 916 & 12514 & 185 & 179\\\hline
		workload error rate (sec. ULM)& [\%] & 7 & 1 & 7 & 6\\\hline
		\end{tabular}

		\caption{{\footnotesize Raw ULMs averaged over 3 repetitions in a network with managed nodes (policy 2). 
}}
	}
	\end{center}
\end{table}
\newpage
\subsection{\label{sec:WL3_NB1}Syn. Varied Weight Workload and Low Churn}

\begin{figure}[h!tpb]
	\centerline{{\footnotesize \resizebox{70mm}{!}{\includegraphics{./appendix/reportFigures/averaged_user-level_metrics.png}}}}
	\caption{\label{fig:Synthetic Varied Weight Workload and Low Membership Churn user-level metrics} mean normalised monitored ULMs averaged over 3 repetitions (NM)}
\end{figure}
\begin{table}[h!tpb]
	\begin{center}
	{\footnotesize
		\begin{tabular}[t]{|l|r|r|r|r|r|}
		\hline user-level metric & unit &  mean & std & median & $1^{st}$ quartile \\\hline
		expected lookup time & [ms] &638 & NA & NA & NA  \\\hline
		network usage& [MB] & 752 & 4 & 754 & 748\\\hline
		workload lookup time (sec. ULM)& [ms] & 638 & 235 & 643 & 461\\\hline
		workload error rate (sec. ULM) & [\%] & 0 & 0 & 0 & 0 \\\hline
		\end{tabular}

		\caption{{\footnotesize Raw ULMs averaged over 3 repetitions in a network with unmanaged nodes. 
}}
		\begin{tabular}[t]{|l|r|r|r|r|r|}
		\hline user-level metric & unit &  mean & std & median & $1^{st}$ quartile \\\hline
		expected lookup time & [ms] &454 & NA & NA & NA  \\\hline
		network usage& [MB] & 77 & 0 & 77 & 77\\\hline
		workload lookup time (sec. ULM)& [ms] & 454 & 152 & 455 & 366\\\hline
		workload error rate (sec. ULM) & [\%] & 0 & 0 & 0 & 0 \\\hline
		\end{tabular}

		\caption{{\footnotesize Raw ULMs averaged over 3 repetitions in a network with managed nodes (policy 1). 
}}
		\begin{tabular}[t]{|l|r|r|r|r|r|}
		\hline user-level metric & unit &  mean & std & median & $1^{st}$ quartile \\\hline
		expected lookup time & [ms] &445 & NA & NA & NA  \\\hline
		network usage& [MB] & 37 & 0 & 37 & 37\\\hline
		workload lookup time (sec. ULM)& [ms] & 445 & 142 & 452 & 363\\\hline
		workload error rate (sec. ULM) & [\%] & 0 & 0 & 0 & 0 \\\hline
		\end{tabular}

		\caption{{\footnotesize Raw ULMs averaged over 3 repetitions in a network with managed nodes (policy 2). 
}}
	}
	\end{center}
\end{table}
\newpage

\subsection{\label{sec:WL3_NB2}Syn. Varied Weight Workload and High Churn}

\begin{figure}[h!tpb]
	\centerline{{\footnotesize \resizebox{70mm}{!}{\includegraphics{./appendix/reportFigures/averaged_user-level_metrics.png}}}}
	\caption{\label{fig:Synthetic Varied Weight Workload and High Membership Churn user-level metrics} mean normalised monitored ULMs averaged over 3 repetitions (NM)}
\end{figure}
\begin{table}[h!tpb]
	\begin{center}
	{\footnotesize
		\begin{tabular}[t]{|l|r|r|r|r|r|}
		\hline user-level metric & unit &  mean & std & median & $1^{st}$ quartile \\\hline
		expected lookup time & [ms] &1089 & NA & NA & NA  \\\hline
		network usage& [MB] & 183 & 207 & 125 & 11\\\hline
		workload lookup time (sec. ULM)& [ms] & 566 & 277 & 555 & 373\\\hline
		time until lookup failed (sec. ULM)& [ms] & 243 & 3572 & 102 & 97\\\hline
		workload error rate (sec. ULM)& [\%] & 50 & 42 & 60 & 4\\\hline
		\end{tabular}

		\caption{{\footnotesize Raw ULMs averaged over 3 repetitions in a network with unmanaged nodes. 
}}
		\begin{tabular}[t]{|l|r|r|r|r|r|}
		\hline user-level metric & unit &  mean & std & median & $1^{st}$ quartile \\\hline
		expected lookup time & [ms] &423 & NA & NA & NA  \\\hline
		network usage& [MB] & 227 & 8 & 231 & 218\\\hline
		workload lookup time (sec. ULM)& [ms] & 405 & 194 & 371 & 274\\\hline
		time until lookup failed (sec. ULM)& [ms] & 122 & 105 & 87 & 85\\\hline
		workload error rate (sec. ULM)& [\%] & 10 & 5 & 12 & 4\\\hline
		\end{tabular}

		\caption{{\footnotesize Raw ULMs averaged over 3 repetitions in a network with managed nodes (policy 1). 
}}
		\begin{tabular}[t]{|l|r|r|r|r|r|}
		\hline user-level metric & unit &  mean & std & median & $1^{st}$ quartile \\\hline
		expected lookup time & [ms] &423 & NA & NA & NA  \\\hline
		network usage& [MB] & 147 & 19 & 144 & 130\\\hline
		workload lookup time (sec. ULM)& [ms] & 389 & 202 & 354 & 244\\\hline
		time until lookup failed (sec. ULM)& [ms] & 174 & 106 & 183 & 86\\\hline
		workload error rate (sec. ULM)& [\%] & 13 & 3 & 15 & 10\\\hline
		\end{tabular}

		\caption{{\footnotesize Raw ULMs averaged over 3 repetitions in a network with managed nodes (policy 2). 
}}
	}
	\end{center}
\end{table}
\newpage

\subsection{\label{sec:WL3_NB3}Syn. Varied Weight Workload and Locally Varying Churn}

\begin{figure}[h!tpb]
	\centerline{{\footnotesize \resizebox{70mm}{!}{\includegraphics{./appendix/reportFigures/averaged_user-level_metrics.png}}}}
	\caption{\label{fig:Synthetic Varied Weight Workload and Locally Varying Membership Churn user-level metrics} mean normalised monitored ULMs averaged over 3 repetitions (NM)}
\end{figure}
\begin{table}[h!tpb]
	\begin{center}
	{\tiny
		\begin{tabular}[t]{|l|r|r|r|r|r|}
		\hline user-level metric & unit &  mean & std & median & $1^{st}$ quartile \\\hline
		expected lookup time & [ms] &580 & NA & NA & NA  \\\hline
		network usage& [MB] & 496 & 3 & 498 & 492\\\hline
		workload lookup time (sec. ULM)& [ms] & 570 & 267 & 551 & 367\\\hline
		time until lookup failed (sec. ULM)& [ms] & 966 & 1021 & 389 & 195\\\hline
		workload error rate (sec. ULM)& [\%] & 1 & 1 & 1 & 1\\\hline
		\end{tabular}

		\caption{{\footnotesize Raw ULMs averaged over 3 repetitions in a network with unmanaged nodes. 
}}
		\begin{tabular}[t]{|l|r|r|r|r|r|}
		\hline user-level metric & unit &  mean & std & median & $1^{st}$ quartile \\\hline
		expected lookup time & [ms] &880 & NA & NA & NA  \\\hline
		network usage& [MB] & 231 & 9 & 227 & 225\\\hline
		workload lookup time (sec. ULM)& [ms] & 444 & 200 & 427 & 282\\\hline
		time until lookup failed (sec. ULM)& [ms] & 6804 & 34634 & 188 & 143\\\hline
		workload error rate (sec. ULM)& [\%] & 6 & 0 & 6 & 5\\\hline
		\end{tabular}

		\caption{{\footnotesize Raw ULMs averaged over 3 repetitions in a network with managed nodes (policy 1). 
}}
		\begin{tabular}[t]{|l|r|r|r|r|r|}
		\hline user-level metric & unit &  mean & std & median & $1^{st}$ quartile \\\hline
		expected lookup time & [ms] &1013 & NA & NA & NA  \\\hline
		network usage& [MB] & 234 & 57 & 239 & 175\\\hline
		workload lookup time (sec. ULM)& [ms] & 572 & 477 & 470 & 279\\\hline
		time until lookup failed (sec. ULM)& [ms] & 2413 & 18462 & 183 & 52\\\hline
		workload error rate (sec. ULM)& [\%] & 15 & 8 & 14 & 7\\\hline
		\end{tabular}

		\caption{{\footnotesize Raw ULMs averaged over 3 repetitions in a network with managed nodes (policy 2). 
}}
	}
	\end{center}
\end{table}
\newpage

\subsection{\label{sec:WL3_NB4}Syn. Varied Weight Workload and Locally Varying Churn}

\begin{figure}[h!tpb]
	\centerline{{\footnotesize \resizebox{70mm}{!}{\includegraphics{./appendix/reportFigures/averaged_user-level_metrics.png}}}}
	\caption{\label{fig:Synthetic Varied Weight Workload and Locally Varying Membership Churn user-level metrics} mean normalised monitored ULMs averaged over 3 repetitions (NM)}
\end{figure}
\begin{table}[h!tpb]
	\begin{center}
	{\footnotesize
		\begin{tabular}[t]{|l|r|r|r|r|r|}
		\hline user-level metric & unit &  mean & std & median & $1^{st}$ quartile \\\hline
		expected lookup time & [ms] &577 & NA & NA & NA  \\\hline
		network usage& [MB] & 575 & 3 & 575 & 572\\\hline
		workload lookup time (sec. ULM)& [ms] & 575 & 257 & 552 & 390\\\hline
		time until lookup failed (sec. ULM)& [ms] & 162 & 144 & 143 & 49\\\hline
		workload error rate (sec. ULM)& [\%] & 1 & 0 & 1 & 1\\\hline
		\end{tabular}

		\caption{{\footnotesize Raw ULMs averaged over 3 repetitions in a network with unmanaged nodes. 
}}
		\begin{tabular}[t]{|l|r|r|r|r|r|}
		\hline user-level metric & unit &  mean & std & median & $1^{st}$ quartile \\\hline
		expected lookup time & [ms] &874 & NA & NA & NA  \\\hline
		network usage& [MB] & 166 & 11 & 161 & 158\\\hline
		workload lookup time (sec. ULM)& [ms] & 435 & 168 & 418 & 312\\\hline
		time until lookup failed (sec. ULM)& [ms] & 8327 & 103703 & 86 & 85\\\hline
		workload error rate (sec. ULM)& [\%] & 5 & 6 & 3 & 2\\\hline
		\end{tabular}

		\caption{{\footnotesize Raw ULMs averaged over 3 repetitions in a network with managed nodes (policy 1). 
}}
		\begin{tabular}[t]{|l|r|r|r|r|r|}
		\hline user-level metric & unit &  mean & std & median & $1^{st}$ quartile \\\hline
		expected lookup time & [ms] &542 & NA & NA & NA  \\\hline
		network usage& [MB] & 141 & 36 & 159 & 99\\\hline
		workload lookup time (sec. ULM)& [ms] & 479 & 186 & 461 & 362\\\hline
		time until lookup failed (sec. ULM)& [ms] & 252 & 725 & 224 & 181\\\hline
		workload error rate (sec. ULM)& [\%] & 16 & 4 & 18 & 12\\\hline
		\end{tabular}

		\caption{{\footnotesize Raw ULMs averaged over 3 repetitions in a network with managed nodes (policy 2). 
}}
	}
	\end{center}
\end{table}
\newpage
\subsection{\label{sec:WL4_NB1}File System Workload and Low Churn}

\begin{figure}[h!tpb]
	\centerline{{\footnotesize \resizebox{70mm}{!}{\includegraphics{./appendix/reportFigures/averaged_user-level_metrics.png}}}}
	\caption{\label{fig:File System Workload and Low Membership Churn user-level metrics} mean normalised monitored ULMs averaged over 3 repetitions (NM)}
\end{figure}
\begin{table}[h!tpb]
	\begin{center}
	{\footnotesize
		\begin{tabular}[t]{|l|r|r|r|r|r|}
		\hline user-level metric & unit &  mean & std & median & $1^{st}$ quartile \\\hline
		expected lookup time & [ms] &876 & NA & NA & NA  \\\hline
		network usage& [MB] & 1400 & 27 & 1394 & 1377\\\hline
		workload lookup time (sec. ULM)& [ms] & 876 & 314 & 899 & 655\\\hline
		time until lookup failed (sec. ULM)& [ms] & 78 & 0 & 78 & 78\\\hline
		workload error rate (sec. ULM)& [\%] & 0 & 0 & 0 & 0\\\hline
		\end{tabular}

		\caption{{\footnotesize Raw ULMs averaged over 3 repetitions in a network with unmanaged nodes. 
}}
		\begin{tabular}[t]{|l|r|r|r|r|r|}
		\hline user-level metric & unit &  mean & std & median & $1^{st}$ quartile \\\hline
		expected lookup time & [ms] &705 & NA & NA & NA  \\\hline
		network usage& [MB] & 365 & 0 & 365 & 365\\\hline
		workload lookup time (sec. ULM)& [ms] & 705 & 244 & 742 & 541\\\hline
		workload error rate (sec. ULM) & [\%] & 0 & 0 & 0 & 0 \\\hline
		\end{tabular}

		\caption{{\footnotesize Raw ULMs averaged over 3 repetitions in a network with managed nodes (policy 1). 
}}
		\begin{tabular}[t]{|l|r|r|r|r|r|}
		\hline user-level metric & unit &  mean & std & median & $1^{st}$ quartile \\\hline
		expected lookup time & [ms] &690 & NA & NA & NA  \\\hline
		network usage& [MB] & 306 & 0 & 306 & 306\\\hline
		workload lookup time (sec. ULM)& [ms] & 690 & 238 & 726 & 530\\\hline
		workload error rate (sec. ULM) & [\%] & 0 & 0 & 0 & 0 \\\hline
		\end{tabular}

		\caption{{\footnotesize Raw ULMs averaged over 3 repetitions in a network with managed nodes (policy 2). 
}}
	}
	\end{center}
\end{table}
\newpage

\subsection{\label{sec:WL4_NB2}File System Workload and High Churn}

\begin{figure}[h!tpb]
	\centerline{{\footnotesize \resizebox{70mm}{!}{\includegraphics{./appendix/reportFigures/averaged_user-level_metrics.png}}}}
	\caption{\label{fig:File System Workload and High Membership Churn user-level metrics} mean normalised monitored ULMs averaged over 3 repetitions (NM)}
\end{figure}
\begin{table}[h!tpb]
	\begin{center}
	{\footnotesize
		\begin{tabular}[t]{|l|r|r|r|r|r|}
		\hline user-level metric & unit &  mean & std & median & $1^{st}$ quartile \\\hline
		expected lookup time & [ms] &838 & NA & NA & NA  \\\hline
		network usage& [MB] & 580 & 323 & 763 & 207\\\hline
		workload lookup time (sec. ULM)& [ms] & 726 & 341 & 715 & 506\\\hline
		time until lookup failed (sec. ULM)& [ms] & 129 & 341 & 89 & 64\\\hline
		workload error rate (sec. ULM)& [\%] & 26 & 41 & 3 & 3\\\hline
		\end{tabular}

		\caption{{\footnotesize Raw ULMs averaged over 3 repetitions in a network with unmanaged nodes. 
}}
		\begin{tabular}[t]{|l|r|r|r|r|r|}
		\hline user-level metric & unit &  mean & std & median & $1^{st}$ quartile \\\hline
		expected lookup time & [ms] &2031 & NA & NA & NA  \\\hline
		network usage& [MB] & 985 & 395 & 1212 & 529\\\hline
		workload lookup time (sec. ULM)& [ms] & 1497 & 1970 & 732 & 506\\\hline
		time until lookup failed (sec. ULM)& [ms] & 3736 & 205918 & 142 & 80\\\hline
		workload error rate (sec. ULM)& [\%] & 12 & 13 & 5 & 4\\\hline
		\end{tabular}

		\caption{{\footnotesize Raw ULMs averaged over 3 repetitions in a network with managed nodes (policy 1). 
}}
		\begin{tabular}[t]{|l|r|r|r|r|r|}
		\hline user-level metric & unit &  mean & std & median & $1^{st}$ quartile \\\hline
		expected lookup time & [ms] &834 & NA & NA & NA  \\\hline
		network usage& [MB] & 272 & 186 & 374 & 57\\\hline
		workload lookup time (sec. ULM)& [ms] & 609 & 271 & 616 & 418\\\hline
		time until lookup failed (sec. ULM)& [ms] & 230 & 3153 & 118 & 72\\\hline
		workload error rate (sec. ULM)& [\%] & 34 & 41 & 13 & 8\\\hline
		\end{tabular}

		\caption{{\footnotesize Raw ULMs averaged over 3 repetitions in a network with managed nodes (policy 2). 
}}
	}
	\end{center}
\end{table}
\newpage

\subsection{\label{sec:WL4_NB3}File System Workload and Locally Varying Churn}

\begin{figure}[h!tpb]
	\centerline{{\footnotesize \resizebox{70mm}{!}{\includegraphics{./appendix/reportFigures/averaged_user-level_metrics.png}}}}
	\caption{\label{fig:File System Workload and Locally Varying Membership Churn user-level metrics} mean normalised monitored ULMs averaged over 3 repetitions (NM)}
\end{figure}
\begin{table}[h!tpb]
	\begin{center}
	{\footnotesize
		\begin{tabular}[t]{|l|r|r|r|r|r|}
		\hline user-level metric & unit &  mean & std & median & $1^{st}$ quartile \\\hline
		expected lookup time & [ms] &2366 & NA & NA & NA  \\\hline
		network usage& [MB] & 1838 & 659 & 1652 & 1292\\\hline
		workload lookup time (sec. ULM)& [ms] & 1821 & 1991 & 925 & 591\\\hline
		time until lookup failed (sec. ULM)& [ms] & 6117 & 28939 & 449 & 191\\\hline
		workload error rate (sec. ULM)& [\%] & 8 & 8 & 5 & 3\\\hline
		\end{tabular}

		\caption{{\footnotesize Raw ULMs averaged over 3 repetitions in a network with unmanaged nodes. 
}}
		\begin{tabular}[t]{|l|r|r|r|r|r|}
		\hline user-level metric & unit &  mean & std & median & $1^{st}$ quartile \\\hline
		expected lookup time & [ms] &1651 & NA & NA & NA  \\\hline
		network usage& [MB] & 519 & 195 & 613 & 295\\\hline
		workload lookup time (sec. ULM)& [ms] & 1053 & 946 & 759 & 529\\\hline
		time until lookup failed (sec. ULM)& [ms] & 2027 & 15234 & 368 & 90\\\hline
		workload error rate (sec. ULM)& [\%] & 21 & 22 & 9 & 8\\\hline
		\end{tabular}

		\caption{{\footnotesize Raw ULMs averaged over 3 repetitions in a network with managed nodes (policy 1). 
}}
		\begin{tabular}[t]{|l|r|r|r|r|r|}
		\hline user-level metric & unit &  mean & std & median & $1^{st}$ quartile \\\hline
		expected lookup time & [ms] &1340 & NA & NA & NA  \\\hline
		network usage& [MB] & 854 & 285 & 708 & 672\\\hline
		workload lookup time (sec. ULM)& [ms] & 798 & 571 & 709 & 453\\\hline
		time until lookup failed (sec. ULM)& [ms] & 2716 & 21396 & 360 & 99\\\hline
		workload error rate (sec. ULM)& [\%] & 16 & 11 & 12 & 7\\\hline
		\end{tabular}

		\caption{{\footnotesize Raw ULMs averaged over 3 repetitions in a network with managed nodes (policy 2). 
}}
	}
	\end{center}
\end{table}
\newpage

\subsection{\label{sec:WL4_NB4}File System Workload and Locally Varying Churn}

\begin{figure}[h!tpb]
	\centerline{{\footnotesize \resizebox{70mm}{!}{\includegraphics{./appendix/reportFigures/averaged_user-level_metrics.png}}}}
	\caption{\label{fig:File System Workload and Locally Varying Membership Churn user-level metrics} mean normalised monitored ULMs averaged over 3 repetitions (NM)}
\end{figure}
\begin{table}[h!tpb]
	\begin{center}
	{\footnotesize
		\begin{tabular}[t]{|l|r|r|r|r|r|}
		\hline user-level metric & unit &  mean & std & median & $1^{st}$ quartile \\\hline
		expected lookup time & [ms] &785 & NA & NA & NA  \\\hline
		network usage& [MB] & 904 & 157 & 979 & 723\\\hline
		workload lookup time (sec. ULM)& [ms] & 770 & 322 & 783 & 551\\\hline
		time until lookup failed (sec. ULM)& [ms] & 114 & 232 & 54 & 47\\\hline
		workload error rate (sec. ULM)& [\%] & 8 & 11 & 1 & 1\\\hline
		\end{tabular}

		\caption{{\footnotesize Raw ULMs averaged over 3 repetitions in a network with unmanaged nodes. 
}}
		\begin{tabular}[t]{|l|r|r|r|r|r|}
		\hline user-level metric & unit &  mean & std & median & $1^{st}$ quartile \\\hline
		expected lookup time & [ms] &673 & NA & NA & NA  \\\hline
		network usage& [MB] & 458 & 21 & 459 & 435\\\hline
		workload lookup time (sec. ULM)& [ms] & 654 & 263 & 669 & 471\\\hline
		time until lookup failed (sec. ULM)& [ms] & 330 & 258 & 327 & 211\\\hline
		workload error rate (sec. ULM)& [\%] & 5 & 1 & 5 & 4\\\hline
		\end{tabular}

		\caption{{\footnotesize Raw ULMs averaged over 3 repetitions in a network with managed nodes (policy 1). 
}}
		\begin{tabular}[t]{|l|r|r|r|r|r|}
		\hline user-level metric & unit &  mean & std & median & $1^{st}$ quartile \\\hline
		expected lookup time & [ms] &713 & NA & NA & NA  \\\hline
		network usage& [MB] & 361 & 46 & 342 & 328\\\hline
		workload lookup time (sec. ULM)& [ms] & 608 & 273 & 617 & 388\\\hline
		time until lookup failed (sec. ULM)& [ms] & 1002 & 25285 & 282 & 145\\\hline
		workload error rate (sec. ULM)& [\%] & 9 & 4 & 7 & 6\\\hline
		\end{tabular}

		\caption{{\footnotesize Raw ULMs averaged over 3 repetitions in a network with managed nodes (policy 2). 
}}
	}
	\end{center}
\end{table}
