# Supplementary material for: Autonomic Management in a Distributed Storage System
Source: arXiv:1007.0328 source file (2010-07-02)
Supplement: Supplementary file 4 [file p2p_preliminary_results.tex]

Here, the detailed results for preliminary series of experiments reported in \ref{Preliminary Experiments:Sampling the Policy Parameter Space} are shown. 
For each series of experiments figures are plotted indicating the effect of the specific policy parameter set on the specific ULM values in the specific experiments, additionally a table shows the extracted ranking metrics. 
All ULM values are normalised in respect to the corresponding values measured in experiments in which nodes were managed with \emph{policy parameter set 0}. The raw ULM values of these experiments are shown in table \ref{tab:raw_data_policy_space_walk}:
\begin{table}[ht!]
\begin{center}
\begin{tabular}{|l|r|r|}
\hline ULM & network with high churn & network with low churn \\\hline
lookup time [ms] & 617 & 508 \\ \hline
lookup error rate [\%] & 0 & 4 \\ \hline
network usage [MB] & 890 & 472 \\ \hline
\end{tabular}
\caption{Raw ULM data from experiments with policy parameter set 0.}
\label{tab:raw_data_policy_space_walk}
\end{center}
\end{table}
The monitored ULMs - lookup time, lookup error rate, network usage - are plotted as bars in a figure per series and per experiment. They are averaged over 3 repetitions and normalised (NM). They are displayed as separate bars for each policy parameter set. The figures also indicate the value of the averaged ULMs (avg. NM) by a horizontal line cutting the ULM bars. Additionally the baseline is plotted at the 100\% level, indication the measurements resulting from policy parameter set 0 in the specific experiment. 
Bars which were above a certain height have been cut of for readability reasons.
Such a cut-off is indicated by an upwards arrow ($\uparrow$) at the top of a cut-off bar and the
information about the actual height of the bar.
The avg. NM for each churn pattern and policy parameter set as well as the ranking metric value are displayed in a table following the histogram. 

\newpage
\subsubsection{Series A}
\begin{figure}[htpb]
	\centerline{{\normalsize \resizebox{70mm}{!}{\includegraphics{/user/markus/data/asa/thesis_writing/tex/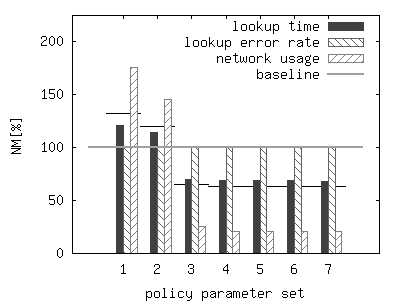}}}}
	\caption{\label{fig:SeriesM NB1}{\normalsize  normalised mean ULMs averaged over 3 repetitions (NM), low  churn }}
	\centerline{{\normalsize \resizebox{70mm}{!}{\includegraphics{/user/markus/data/asa/thesis_writing/tex/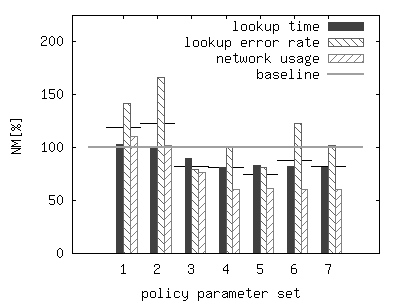}}}}
	\caption{\label{fig:SeriesM NB2}{\normalsize  normalised mean ULMs averaged over 3 repetitions (NM), high  churn }}
\end{figure}
\begin{table}[htpb]
	\begin{center}
	{\normalsize
		\begin{tabular}[t]{|l|r|r|r|}
		\hline policy parameter set & avg. NM - low  churn & avg. NM - high  churn & ranking metric \\\hline
policy1 & 132 & 119 & 126\\\hline
policy2 & 120 & 123 & 122\\\hline
policy3 & 65 & 82 & 74\\\hline
policy4 & 63 & 81 & 72\\\hline
policy5 & 63 & 75 & 69\\\hline
policy6 & 63 & 88 & 76\\\hline
policy7 & 63 & 82 & 73\\\hline
		\end{tabular}

		\caption{{\normalsize  averaged NM (ranking metric) }}
	}
	\end{center}
\end{table}
\newpage
\subsubsection{Series B}
\begin{figure}[htpb]
	\centerline{{\normalsize \resizebox{70mm}{!}{\includegraphics{/user/markus/data/asa/thesis_writing/tex/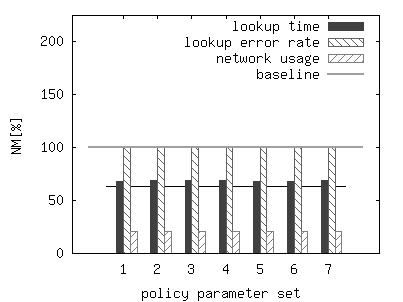}}}}
	\caption{\label{fig:SeriesN NB1}{\normalsize  normalised mean ULMs averaged over 3 repetitions (NM), low  churn }}
	\centerline{{\normalsize \resizebox{70mm}{!}{\includegraphics{/user/markus/data/asa/thesis_writing/tex/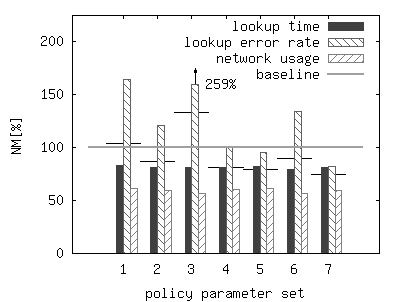}}}}
	\caption{\label{fig:SeriesN NB2}{\normalsize  normalised mean ULMs averaged over 3 repetitions (NM), high  churn }}
\end{figure}
\begin{table}[htpb]
	\begin{center}
	{\normalsize
		\begin{tabular}[t]{|l|r|r|r|}
		\hline policy parameter set & avg. NM - low  churn & avg. NM - high  churn & ranking metric \\\hline
policy1 & 63 & 104 & 84\\\hline
policy2 & 63 & 87 & 75\\\hline
policy3 & 63 & 133 & 98\\\hline
policy4 & 63 & 81 & 72\\\hline
policy5 & 63 & 79 & 71\\\hline
policy6 & 63 & 90 & 77\\\hline
policy7 & 63 & 75 & 69\\\hline
		\end{tabular}

		\caption{{\normalsize  averaged NM (ranking metric) }}
	}
	\end{center}
\end{table}
\newpage
\subsubsection{Series C}
\begin{figure}[htpb]
	\centerline{{\normalsize \resizebox{70mm}{!}{\includegraphics{/user/markus/data/asa/thesis_writing/tex/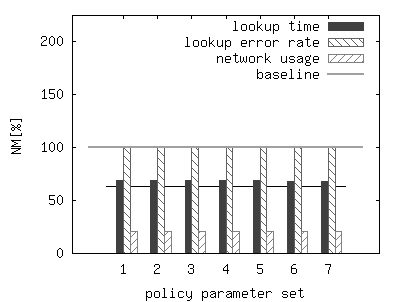}}}}
	\caption{\label{fig:SeriesO NB1}{\normalsize  normalised mean ULMs averaged over 3 repetitions (NM), low  churn }}
	\centerline{{\normalsize \resizebox{70mm}{!}{\includegraphics{/user/markus/data/asa/thesis_writing/tex/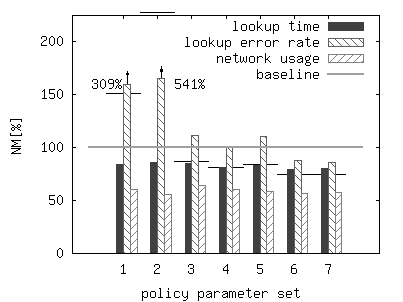}}}}
	\caption{\label{fig:SeriesO NB2}{\normalsize  normalised mean ULMs averaged over 3 repetitions (NM), high  churn }}
\end{figure}
\begin{table}[htpb]
	\begin{center}
	{\normalsize
		\begin{tabular}[t]{|l|r|r|r|}
		\hline policy parameter set & avg. NM - low  churn & avg. NM - high  churn & ranking metric \\\hline
policy1 & 63 & 151 & 107\\\hline
policy2 & 63 & 228 & 146\\\hline
policy3 & 63 & 87 & 75\\\hline
policy4 & 63 & 81 & 72\\\hline
policy5 & 63 & 84 & 74\\\hline
policy6 & 63 & 75 & 69\\\hline
policy7 & 63 & 75 & 69\\\hline
		\end{tabular}

		\caption{{\normalsize  averaged NM (ranking metric) }}
	}
	\end{center}
\end{table}
\newpage
\subsubsection{Series D}
\begin{figure}[htpb]
	\centerline{{\normalsize \resizebox{70mm}{!}{\includegraphics{/user/markus/data/asa/thesis_writing/tex/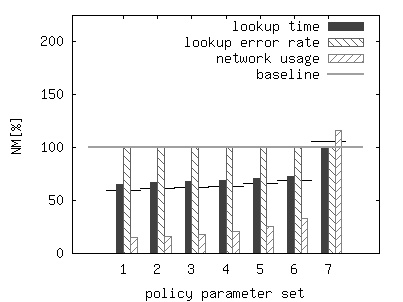}}}}
	\caption{\label{fig:SeriesP NB1}{\normalsize  normalised mean ULMs averaged over 3 repetitions (NM), low  churn }}
	\centerline{{\normalsize \resizebox{70mm}{!}{\includegraphics{/user/markus/data/asa/thesis_writing/tex/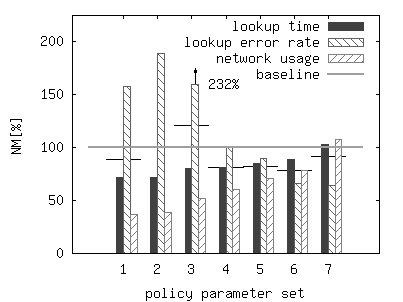}}}}
	\caption{\label{fig:SeriesP NB2}{\normalsize  normalised mean ULMs averaged over 3 repetitions (NM), high  churn }}
\end{figure}
\begin{table}[htpb]
	\begin{center}
	{\normalsize
		\begin{tabular}[t]{|l|r|r|r|}
		\hline policy parameter set & avg. NM - low  churn & avg. NM - high  churn & ranking metric \\\hline
policy1 & 60 & 89 & 75\\\hline
policy2 & 61 & 100 & 81\\\hline
policy3 & 62 & 121 & 92\\\hline
policy4 & 63 & 81 & 72\\\hline
policy5 & 66 & 82 & 74\\\hline
policy6 & 69 & 78 & 74\\\hline
policy7 & 106 & 92 & 99\\\hline
		\end{tabular}

		\caption{{\normalsize  averaged NM (ranking metric) }}
	}
	\end{center}
\end{table}
\newpage
\subsubsection{Series E}
\begin{figure}[htpb]
	\centerline{{\normalsize \resizebox{70mm}{!}{\includegraphics{/user/markus/data/asa/thesis_writing/tex/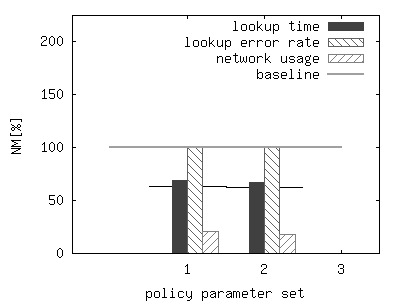}}}}
	\caption{\label{fig:SeriesQ NB1}{\normalsize  normalised mean ULMs averaged over 3 repetitions (NM), low  churn }}
	\centerline{{\normalsize \resizebox{70mm}{!}{\includegraphics{/user/markus/data/asa/thesis_writing/tex/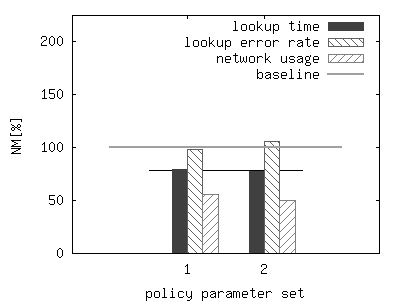}}}}
	\caption{\label{fig:SeriesQ NB2}{\normalsize  normalised mean ULMs averaged over 3 repetitions (NM), high  churn }}
\end{figure}
\begin{table}[htpb]
	\begin{center}
	{\normalsize
		\begin{tabular}[t]{|l|r|r|r|}
		\hline policy parameter set & avg. NM - low  churn & avg. NM - high  churn & ranking metric \\\hline
policy1 & 63 & 78 & 71\\\hline
policy2 & 62 & 78 & 70\\\hline
		\end{tabular}

		\caption{{\normalsize  averaged NM (ranking metric) }}
	}
	\end{center}
\end{table}
\newpage

\newpage
