# Supplementary material for: Autonomic Management in a Distributed Storage System
Source: arXiv:1007.0328 source file (2010-07-02)
Supplement: Supplementary file 9 [file abbreviations.tex]

\begin{table}[h!]
\begin{center}
\begin{tabular}{|c|l|}
\hline
abbreviation & description \\\hline
CP1 & low churn \\\hline
CP2 & high churn \\\hline
CP3 & temporally varying churn \\\hline
WL1 & heavy weight workload \\\hline
WL2 & light weight workload \\\hline
WL3 & temporally varying workload \\\hline
DS1 & big data item size \\\hline
DS2 & small data item size \\\hline
\end{tabular}
\caption{Abbreviations}
%i.e. how often AM won vs. NO management 
\label{tab:abbreviations1}
\end{center}
\end{table}
