# Supplementary material for: Autonomic Management in a Distributed Storage System
Source: arXiv:1007.0328 source file (2010-07-02)
Supplement: Supplementary file 10 [file policySpaceWalkSummary.tex]

\subsubsection{Series A}
\begin{figure}[htpb]
	\centerline{{\normalsize \resizebox{70mm}{!}{\includegraphics{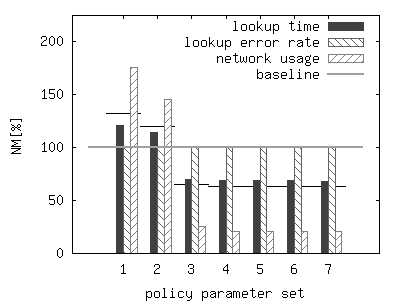}}}}
	\caption{\label{fig:SeriesM NB1}{\normalsize  normalised mean ULMs averaged over 3 repetitions (NM), low  churn }}
	\centerline{{\normalsize \resizebox{70mm}{!}{\includegraphics{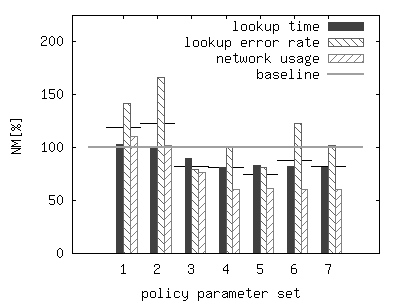}}}}
	\caption{\label{fig:SeriesM NB2}{\normalsize  normalised mean ULMs averaged over 3 repetitions (NM), high  churn }}
\end{figure}
\begin{table}[htpb]
	\begin{center}
	{\normalsize
		\begin{tabular}[t]{|l|r|r|r|}
		\hline policy parameter set & avg. NM - low  churn & avg. NM - high  churn & ranking metric \\\hline
policy1 & 132 & 119 & 126\\\hline
policy2 & 120 & 123 & 122\\\hline
policy3 & 65 & 82 & 74\\\hline
policy4 & 63 & 81 & 72\\\hline
policy5 & 63 & 75 & 69\\\hline
policy6 & 63 & 88 & 76\\\hline
policy7 & 63 & 82 & 73\\\hline
		\end{tabular}

		\caption{{\normalsize  averaged NM (ranking metric) }}
	}
	\end{center}
\end{table}
\newpage
\subsubsection{Series B}
\begin{figure}[htpb]
	\centerline{{\normalsize \resizebox{70mm}{!}{\includegraphics{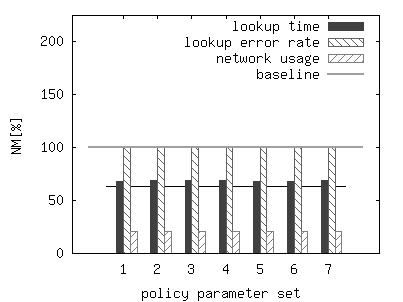}}}}
	\caption{\label{fig:SeriesN NB1}{\normalsize  normalised mean ULMs averaged over 3 repetitions (NM), low  churn }}
	\centerline{{\normalsize \resizebox{70mm}{!}{\includegraphics{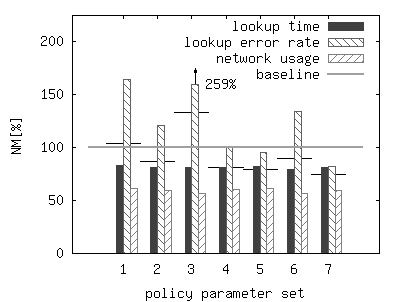}}}}
	\caption{\label{fig:SeriesN NB2}{\normalsize  normalised mean ULMs averaged over 3 repetitions (NM), high  churn }}
\end{figure}
\begin{table}[htpb]
	\begin{center}
	{\normalsize
		\begin{tabular}[t]{|l|r|r|r|}
		\hline policy parameter set & avg. NM - low  churn & avg. NM - high  churn & ranking metric \\\hline
policy1 & 63 & 104 & 84\\\hline
policy2 & 63 & 87 & 75\\\hline
policy3 & 63 & 133 & 98\\\hline
policy4 & 63 & 81 & 72\\\hline
policy5 & 63 & 79 & 71\\\hline
policy6 & 63 & 90 & 77\\\hline
policy7 & 63 & 75 & 69\\\hline
		\end{tabular}

		\caption{{\normalsize  averaged NM (ranking metric) }}
	}
	\end{center}
\end{table}
\newpage
\subsubsection{Series C}
\begin{figure}[htpb]
	\centerline{{\normalsize \resizebox{70mm}{!}{\includegraphics{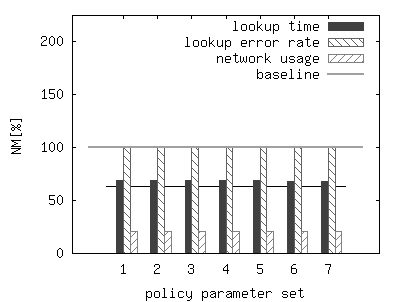}}}}
	\caption{\label{fig:SeriesO NB1}{\normalsize  normalised mean ULMs averaged over 3 repetitions (NM), low  churn }}
	\centerline{{\normalsize \resizebox{70mm}{!}{\includegraphics{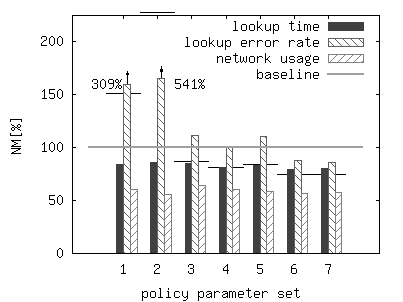}}}}
	\caption{\label{fig:SeriesO NB2}{\normalsize  normalised mean ULMs averaged over 3 repetitions (NM), high  churn }}
\end{figure}
\begin{table}[htpb]
	\begin{center}
	{\normalsize
		\begin{tabular}[t]{|l|r|r|r|}
		\hline policy parameter set & avg. NM - low  churn & avg. NM - high  churn & ranking metric \\\hline
policy1 & 63 & 151 & 107\\\hline
policy2 & 63 & 228 & 146\\\hline
policy3 & 63 & 87 & 75\\\hline
policy4 & 63 & 81 & 72\\\hline
policy5 & 63 & 84 & 74\\\hline
policy6 & 63 & 75 & 69\\\hline
policy7 & 63 & 75 & 69\\\hline
		\end{tabular}

		\caption{{\normalsize  averaged NM (ranking metric) }}
	}
	\end{center}
\end{table}
\newpage
\subsubsection{Series D}
\begin{figure}[htpb]
	\centerline{{\normalsize \resizebox{70mm}{!}{\includegraphics{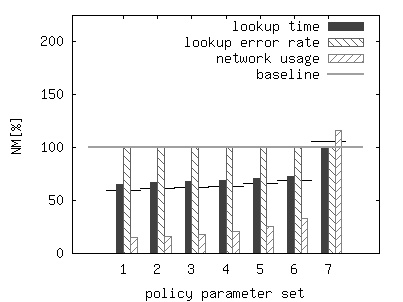}}}}
	\caption{\label{fig:SeriesP NB1}{\normalsize  normalised mean ULMs averaged over 3 repetitions (NM), low  churn }}
	\centerline{{\normalsize \resizebox{70mm}{!}{\includegraphics{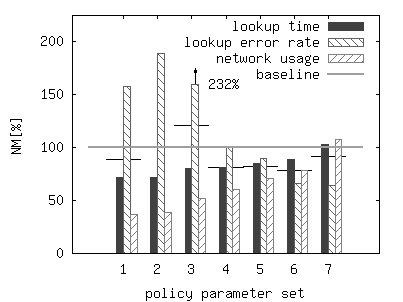}}}}
	\caption{\label{fig:SeriesP NB2}{\normalsize  normalised mean ULMs averaged over 3 repetitions (NM), high  churn }}
\end{figure}
\begin{table}[htpb]
	\begin{center}
	{\normalsize
		\begin{tabular}[t]{|l|r|r|r|}
		\hline policy parameter set & avg. NM - low  churn & avg. NM - high  churn & ranking metric \\\hline
policy1 & 60 & 89 & 75\\\hline
policy2 & 61 & 100 & 81\\\hline
policy3 & 62 & 121 & 92\\\hline
policy4 & 63 & 81 & 72\\\hline
policy5 & 66 & 82 & 74\\\hline
policy6 & 69 & 78 & 74\\\hline
policy7 & 106 & 92 & 99\\\hline
		\end{tabular}

		\caption{{\normalsize  averaged NM (ranking metric) }}
	}
	\end{center}
\end{table}
\newpage
\subsubsection{Series E}
\begin{figure}[htpb]
	\centerline{{\normalsize \resizebox{70mm}{!}{\includegraphics{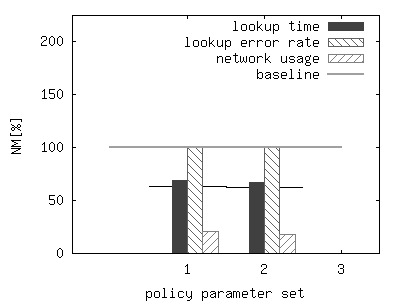}}}}
	\caption{\label{fig:SeriesQ NB1}{\normalsize  normalised mean ULMs averaged over 3 repetitions (NM), low  churn }}
	\centerline{{\normalsize \resizebox{70mm}{!}{\includegraphics{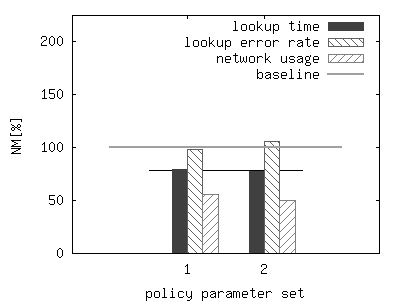}}}}
	\caption{\label{fig:SeriesQ NB2}{\normalsize  normalised mean ULMs averaged over 3 repetitions (NM), high  churn }}
\end{figure}
\begin{table}[htpb]
	\begin{center}
	{\normalsize
		\begin{tabular}[t]{|l|r|r|r|}
		\hline policy parameter set & avg. NM - low  churn & avg. NM - high  churn & ranking metric \\\hline
policy1 & 63 & 78 & 71\\\hline
policy2 & 62 & 78 & 70\\\hline
		\end{tabular}

		\caption{{\normalsize  averaged NM (ranking metric) }}
	}
	\end{center}
\end{table}
\newpage
