# Supplementary material for: Autonomic Management in a Distributed Storage System
Source: arXiv:1007.0328 source file (2010-07-02)
Supplement: Supplementary file 17 [file p2p_main_results_reports.tex]

\newpage

\subsection{\label{appendix::p2p:WL1_NB1}Synthetic Light Weight Workload with Low Churn}

\subsubsection{Summarised Effects of Policies on Expected Lookup Time and Network Usage}
\begin{figure}[htpb]
	\centerline{{\resizebox{95mm}{!}{\includegraphics{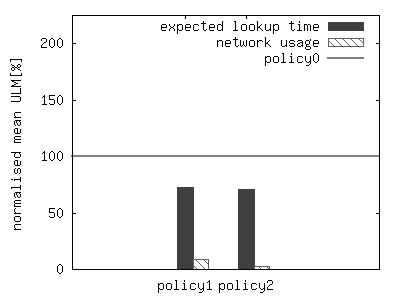}}}}
	\caption{\label{fig:Synthetic Light Weight Workload with Low Churn user-level metrics} normalised mean ULM values}
\end{figure}
		\vspace{5 mm}

\begin{table}[htpb]
	\begin{center}
		\begin{tabular}[t]{|l|r|r|}
		\hline policy & mean expected lookup time [ms] & mean network usage [MB/5 min]  \\\hline
		 policy 0 &  720 & 60\\\hline
		 policy 1 & 522 & 5\\\hline
		 policy 2 & 507 & 2\\\hline
		\end{tabular}

		\caption{\label{tab:ULMWL1_NB1} mean ULM values}
	\end{center}
	\end{table}
\newpage

\subsubsection{Summary of ULM Distributions}
\begin{table}[htpb]
	\begin{center}
		\vspace{10 mm}

		\resizebox{\textwidth}{!}{
		\begin{tabular}[t]{|l||c|c|c|c|c|c|c|c|}
		\hline ULM & unit & $ci_\mu$ & $s$ & min & $Q_1$ & $Q_2$ & $Q_3$ & max \\\hline
		ELT (primary)& [ms] & 720$\pm$62 & 207 & 357 & 516 & 777 & 857 & 1075\\\hline
		NU (primary)& [MB/5 min] & 60$\pm$6 & 20 & 2 & 66 & 66 & 68 & 68\\\hline\hline
		LT (secondary)& [ms] & 720$\pm$62 & 207 & 357 & 516 & 777 & 857 & 1075\\\hline
		LET (secondary) & [ms]  & NA&  NA & NA & NA & NA & NA & NA  \\\hline
		LER (secondary)& [\%] & 0$\pm$0 & 0 & 0 & 0 & 0 & 0 & 0\\\hline
		\end{tabular}}

		\caption{{\normalsize ULM distributions, measured with unmanaged nodes (policy 0). 
}}
		\vspace{10 mm}

		\resizebox{\textwidth}{!}{
		\begin{tabular}[t]{|l||c|c|c|c|c|c|c|c|}
		\hline ULM & unit & $ci_\mu$ & $s$ & min & $Q_1$ & $Q_2$ & $Q_3$ & max \\\hline
		ELT (primary)& [ms] & 522$\pm$43 & 145 & 291 & 406 & 535 & 607 & 875\\\hline
		NU (primary)& [MB/5 min] & 5$\pm$1 & 4 & 0 & 3 & 4 & 7 & 16\\\hline\hline
		LT (secondary)& [ms] & 522$\pm$43 & 145 & 291 & 406 & 535 & 607 & 875\\\hline
		LET (secondary) & [ms]  & NA&  NA & NA & NA & NA & NA & NA  \\\hline
		LER (secondary)& [\%] & 0$\pm$0 & 0 & 0 & 0 & 0 & 0 & 0\\\hline
		\end{tabular}}

		\caption{{\normalsize ULM distributions, measured with managed nodes (policy 1). 
}}
		\vspace{10 mm}

		\resizebox{\textwidth}{!}{
		\begin{tabular}[t]{|l||c|c|c|c|c|c|c|c|}
		\hline ULM & unit & $ci_\mu$ & $s$ & min & $Q_1$ & $Q_2$ & $Q_3$ & max \\\hline
		ELT (primary)& [ms] & 507$\pm$36 & 121 & 291 & 425 & 567 & 606 & 635\\\hline
		NU (primary)& [MB/5 min] & 2$\pm$0 & 1 & 0 & 1 & 1 & 2 & 5\\\hline\hline
		LT (secondary)& [ms] & 507$\pm$36 & 121 & 291 & 425 & 567 & 606 & 635\\\hline
		LET (secondary) & [ms]  & NA&  NA & NA & NA & NA & NA & NA  \\\hline
		LER (secondary)& [\%] & 0$\pm$0 & 0 & 0 & 0 & 0 & 0 & 0\\\hline
		\end{tabular}}

		\caption{{\normalsize ULM distributions, measured with managed nodes (policy 2). 
}}
	\end{center}
\end{table}
\newpage

\subsection{\label{appendix::p2p:WL1_NB2}Synthetic Light Weight Workload with High Churn}

\subsubsection{Summarised Effects of Policies on Expected Lookup Time and Network Usage}
\begin{figure}[htpb]
	\centerline{{\resizebox{95mm}{!}{\includegraphics{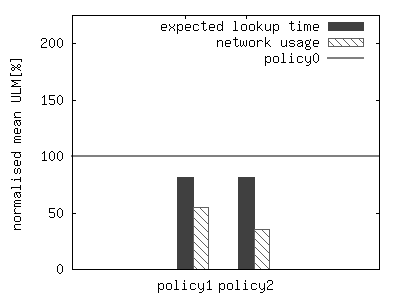}}}}
	\caption{\label{fig:Synthetic Light Weight Workload with High Churn user-level metrics} normalised mean ULM values}
\end{figure}
		\vspace{5 mm}

\begin{table}[htpb]
	\begin{center}
		\begin{tabular}[t]{|l|r|r|}
		\hline policy & mean expected lookup time [ms] & mean network usage [MB/5 min]  \\\hline
		 policy 0 &  562 & 33\\\hline
		 policy 1 & 457 & 18\\\hline
		 policy 2 & 459 & 12\\\hline
		\end{tabular}

		\caption{\label{tab:ULMWL1_NB2} mean ULM values}
	\end{center}
	\end{table}
\newpage

\subsubsection{Summary of ULM Distributions}
\begin{table}[htpb]
	\begin{center}
		\vspace{10 mm}

		\resizebox{\textwidth}{!}{
		\begin{tabular}[t]{|l||c|c|c|c|c|c|c|c|}
		\hline ULM & unit & $ci_\mu$ & $s$ & min & $Q_1$ & $Q_2$ & $Q_3$ & max \\\hline
		ELT (primary)& [ms] & 562$\pm$92 & 296 & 176 & 398 & 551 & 637 & 1710\\\hline
		NU (primary)& [MB/5 min] & 33$\pm$4 & 13 & 0 & 32 & 37 & 40 & 43\\\hline\hline
		LT (secondary)& [ms] & 562$\pm$92 & 296 & 176 & 398 & 551 & 637 & 1710\\\hline
		LET (secondary)& [ms] & 11$\pm$4 & 4 & 8 & 8 & 11 & 13 & 13\\\hline
		LER (secondary)& [\%] & 7$\pm$8 & 25 & 0 & 0 & 0 & 0 & 100\\\hline
		\end{tabular}}

		\caption{{\normalsize ULM distributions, measured with unmanaged nodes (policy 0). 
}}
		\vspace{10 mm}

		\resizebox{\textwidth}{!}{
		\begin{tabular}[t]{|l||c|c|c|c|c|c|c|c|}
		\hline ULM & unit & $ci_\mu$ & $s$ & min & $Q_1$ & $Q_2$ & $Q_3$ & max \\\hline
		ELT (primary)& [ms] & 457$\pm$60 & 166 & 128 & 386 & 482 & 544 & 779\\\hline
		NU (primary)& [MB/5 min] & 18$\pm$2 & 7 & 0 & 17 & 21 & 22 & 23\\\hline\hline
		LT (secondary)& [ms] & 457$\pm$60 & 166 & 128 & 386 & 482 & 544 & 779\\\hline
		LET (secondary)& [ms] & 16493$\pm$27105 & 49431 & 11 & 13 & 17 & 20 & 148308\\\hline
		LER (secondary)& [\%] & 30$\pm$14 & 47 & 0 & 0 & 0 & 100 & 100\\\hline
		\end{tabular}}

		\caption{{\normalsize ULM distributions, measured with managed nodes (policy 1). 
}}
		\vspace{10 mm}

		\resizebox{\textwidth}{!}{
		\begin{tabular}[t]{|l||c|c|c|c|c|c|c|c|}
		\hline ULM & unit & $ci_\mu$ & $s$ & min & $Q_1$ & $Q_2$ & $Q_3$ & max \\\hline
		ELT (primary)& [ms] & 459$\pm$100 & 265 & 149 & 311 & 428 & 527 & 1434\\\hline
		NU (primary)& [MB/5 min] & 12$\pm$1 & 4 & 0 & 9 & 12 & 15 & 17\\\hline\hline
		LT (secondary)& [ms] & 459$\pm$100 & 265 & 149 & 311 & 428 & 527 & 1434\\\hline
		LET (secondary)& [ms] & 12555$\pm$20540 & 41412 & 9 & 13 & 47 & 49 & 137418\\\hline
		LER (secondary)& [\%] & 37$\pm$15 & 49 & 0 & 0 & 0 & 100 & 100\\\hline
		\end{tabular}}

		\caption{{\normalsize ULM distributions, measured with managed nodes (policy 2). 
}}
	\end{center}
\end{table}
\newpage

\subsection{\label{appendix::p2p:WL1_NB3}Synthetic Light Weight Workload with Locally Varying Churn}

\subsubsection{Summarised Effects of Policies on Expected Lookup Time and Network Usage}
\begin{figure}[htpb]
	\centerline{{\resizebox{95mm}{!}{\includegraphics{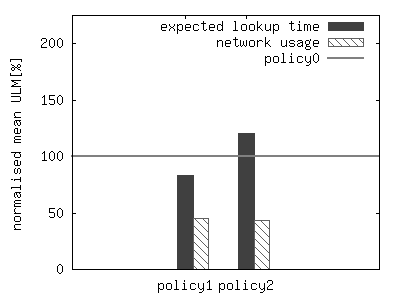}}}}
	\caption{\label{fig:Synthetic Light Weight Workload with Locally Varying Churn user-level metrics} normalised mean ULM values}
\end{figure}
		\vspace{5 mm}

\begin{table}[htpb]
	\begin{center}
		\begin{tabular}[t]{|l|r|r|}
		\hline policy & mean expected lookup time [ms] & mean network usage [MB/5 min]  \\\hline
		 policy 0 &  689 & 40\\\hline
		 policy 1 & 575 & 18\\\hline
		 policy 2 & 831 & 17\\\hline
		\end{tabular}

		\caption{\label{tab:ULMWL1_NB3} mean ULM values}
	\end{center}
	\end{table}
\newpage

\subsubsection{Summary of ULM Distributions}
\begin{table}[htpb]
	\begin{center}
		\vspace{10 mm}

		\resizebox{\textwidth}{!}{
		\begin{tabular}[t]{|l||c|c|c|c|c|c|c|c|}
		\hline ULM & unit & $ci_\mu$ & $s$ & min & $Q_1$ & $Q_2$ & $Q_3$ & max \\\hline
		ELT (primary)& [ms] & 689$\pm$75 & 248 & 137 & 550 & 708 & 830 & 1091\\\hline
		NU (primary)& [MB/5 min] & 40$\pm$4 & 13 & 1 & 41 & 43 & 45 & 49\\\hline\hline
		LT (secondary)& [ms] & 689$\pm$75 & 248 & 137 & 550 & 708 & 830 & 1091\\\hline
		LET (secondary) & [ms]  & NA&  NA & NA & NA & NA & NA & NA  \\\hline
		LER (secondary)& [\%] & 0$\pm$0 & 0 & 0 & 0 & 0 & 0 & 0\\\hline
		\end{tabular}}

		\caption{{\normalsize ULM distributions, measured with unmanaged nodes (policy 0). 
}}
		\vspace{10 mm}

		\resizebox{\textwidth}{!}{
		\begin{tabular}[t]{|l||c|c|c|c|c|c|c|c|}
		\hline ULM & unit & $ci_\mu$ & $s$ & min & $Q_1$ & $Q_2$ & $Q_3$ & max \\\hline
		ELT (primary)& [ms] & 575$\pm$72 & 224 & 151 & 422 & 612 & 712 & 944\\\hline
		NU (primary)& [MB/5 min] & 18$\pm$2 & 7 & 0 & 17 & 19 & 23 & 26\\\hline\hline
		LT (secondary)& [ms] & 575$\pm$72 & 224 & 151 & 422 & 612 & 712 & 944\\\hline
		LET (secondary)& [ms] & 186$\pm$109 & 133 & 10 & 55 & 201 & 301 & 331\\\hline
		LER (secondary)& [\%] & 13$\pm$10 & 35 & 0 & 0 & 0 & 0 & 100\\\hline
		\end{tabular}}

		\caption{{\normalsize ULM distributions, measured with managed nodes (policy 1). 
}}
		\vspace{10 mm}

		\resizebox{\textwidth}{!}{
		\begin{tabular}[t]{|l||c|c|c|c|c|c|c|c|}
		\hline ULM & unit & $ci_\mu$ & $s$ & min & $Q_1$ & $Q_2$ & $Q_3$ & max \\\hline
		ELT (primary)& [ms] & 831$\pm$185 & 574 & 136 & 448 & 701 & 947 & 2122\\\hline
		NU (primary)& [MB/5 min] & 17$\pm$3 & 10 & 0 & 10 & 18 & 25 & 35\\\hline\hline
		LT (secondary)& [ms] & 831$\pm$185 & 574 & 136 & 448 & 701 & 947 & 2122\\\hline
		LET (secondary)& [ms] & 56$\pm$76 & 93 & 9 & 9 & 11 & 149 & 195\\\hline
		LER (secondary)& [\%] & 13$\pm$10 & 35 & 0 & 0 & 0 & 0 & 100\\\hline
		\end{tabular}}

		\caption{{\normalsize ULM distributions, measured with managed nodes (policy 2). 
}}
	\end{center}
\end{table}
\newpage

\subsection{\label{appendix::p2p:WL1_NB4}Synthetic Light Weight Workload with Temporally Varying Churn}

\subsubsection{Summarised Effects of Policies on Expected Lookup Time and Network Usage}
\begin{figure}[htpb]
	\centerline{{\resizebox{95mm}{!}{\includegraphics{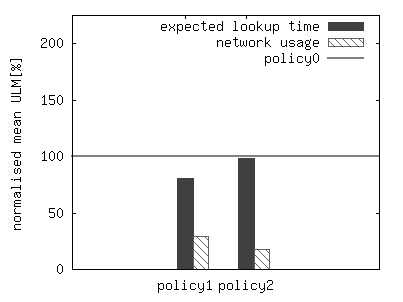}}}}
	\caption{\label{fig:Synthetic Light Weight Workload with Temporally Varying Churn user-level metrics} normalised mean ULM values}
\end{figure}
		\vspace{5 mm}

\begin{table}[htpb]
	\begin{center}
		\begin{tabular}[t]{|l|r|r|}
		\hline policy & mean expected lookup time [ms] & mean network usage [MB/5 min]  \\\hline
		 policy 0 &  643 & 44\\\hline
		 policy 1 & 518 & 13\\\hline
		 policy 2 & 629 & 8\\\hline
		\end{tabular}

		\caption{\label{tab:ULMWL1_NB4} mean ULM values}
	\end{center}
	\end{table}
\newpage

\subsubsection{Summary of ULM Distributions}
\begin{table}[htpb]
	\begin{center}
		\vspace{10 mm}

		\resizebox{\textwidth}{!}{
		\begin{tabular}[t]{|l||c|c|c|c|c|c|c|c|}
		\hline ULM & unit & $ci_\mu$ & $s$ & min & $Q_1$ & $Q_2$ & $Q_3$ & max \\\hline
		ELT (primary)& [ms] & 643$\pm$75 & 232 & 139 & 463 & 602 & 871 & 1077\\\hline
		NU (primary)& [MB/5 min] & 44$\pm$5 & 18 & 1 & 37 & 42 & 60 & 67\\\hline\hline
		LT (secondary)& [ms] & 643$\pm$75 & 232 & 139 & 463 & 602 & 871 & 1077\\\hline
		LET (secondary)& [ms] & 397$\pm$631 & 767 & 13 & 13 & 14 & 1165 & 1548\\\hline
		LER (secondary)& [\%] & 13$\pm$10 & 35 & 0 & 0 & 0 & 0 & 100\\\hline
		\end{tabular}}

		\caption{{\normalsize ULM distributions, measured with unmanaged nodes (policy 0). 
}}
		\vspace{10 mm}

		\resizebox{\textwidth}{!}{
		\begin{tabular}[t]{|l||c|c|c|c|c|c|c|c|}
		\hline ULM & unit & $ci_\mu$ & $s$ & min & $Q_1$ & $Q_2$ & $Q_3$ & max \\\hline
		ELT (primary)& [ms] & 518$\pm$48 & 152 & 308 & 441 & 466 & 604 & 935\\\hline
		NU (primary)& [MB/5 min] & 13$\pm$2 & 6 & 0 & 9 & 14 & 17 & 22\\\hline\hline
		LT (secondary)& [ms] & 518$\pm$48 & 152 & 308 & 441 & 466 & 604 & 935\\\hline
		LET (secondary)& [ms] & 12$\pm$0 & 0 & 12 & 12 & 12 & 12 & 12\\\hline
		LER (secondary)& [\%] & 10$\pm$9 & 31 & 0 & 0 & 0 & 0 & 100\\\hline
		\end{tabular}}

		\caption{{\normalsize ULM distributions, measured with managed nodes (policy 1). 
}}
		\vspace{10 mm}

		\resizebox{\textwidth}{!}{
		\begin{tabular}[t]{|l||c|c|c|c|c|c|c|c|}
		\hline ULM & unit & $ci_\mu$ & $s$ & min & $Q_1$ & $Q_2$ & $Q_3$ & max \\\hline
		ELT (primary)& [ms] & 629$\pm$162 & 503 & 152 & 311 & 466 & 680 & 2039\\\hline
		NU (primary)& [MB/5 min] & 8$\pm$2 & 5 & 0 & 4 & 7 & 12 & 18\\\hline\hline
		LT (secondary)& [ms] & 629$\pm$162 & 503 & 152 & 311 & 466 & 680 & 2039\\\hline
		LET (secondary)& [ms] & 15855$\pm$15113 & 18374 & 8 & 9 & 14820 & 32735 & 33771\\\hline
		LER (secondary)& [\%] & 13$\pm$10 & 35 & 0 & 0 & 0 & 0 & 100\\\hline
		\end{tabular}}

		\caption{{\normalsize ULM distributions, measured with managed nodes (policy 2). 
}}
	\end{center}
\end{table}
\newpage

\subsection{\label{appendix::p2p:WL2_NB1}Synthetic Heavy Weight Workload with Low Churn}

\subsubsection{Summarised Effects of Policies on Expected Lookup Time and Network Usage}
\begin{figure}[htpb]
	\centerline{{\resizebox{95mm}{!}{\includegraphics{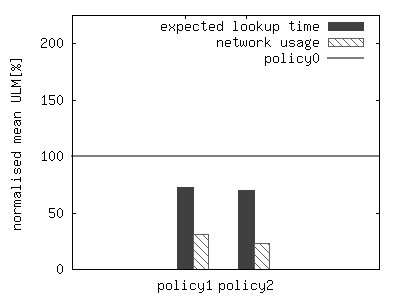}}}}
	\caption{\label{fig:Synthetic Heavy Weight Workload with Low Churn user-level metrics} normalised mean ULM values}
\end{figure}
		\vspace{5 mm}

\begin{table}[htpb]
	\begin{center}
		\begin{tabular}[t]{|l|r|r|}
		\hline policy & mean expected lookup time [ms] & mean network usage [MB/5 min]  \\\hline
		 policy 0 &  613 & 69\\\hline
		 policy 1 & 445 & 22\\\hline
		 policy 2 & 428 & 16\\\hline
		\end{tabular}

		\caption{\label{tab:ULMWL2_NB1} mean ULM values}
	\end{center}
	\end{table}
\newpage

\subsubsection{Summary of ULM Distributions}
\begin{table}[htpb]
	\begin{center}
		\vspace{10 mm}

		\resizebox{\textwidth}{!}{
		\begin{tabular}[t]{|l||c|c|c|c|c|c|c|c|}
		\hline ULM & unit & $ci_\mu$ & $s$ & min & $Q_1$ & $Q_2$ & $Q_3$ & max \\\hline
		ELT (primary)& [ms] & 613$\pm$7 & 25 & 538 & 611 & 619 & 627 & 640\\\hline
		NU (primary)& [MB/5 min] & 69$\pm$4 & 15 & 17 & 73 & 74 & 74 & 75\\\hline\hline
		LT (secondary)& [ms] & 613$\pm$3 & 228 & 89 & 444 & 615 & 774 & 2505\\\hline
		LET (secondary) & [ms]  & NA&  NA & NA & NA & NA & NA & NA  \\\hline
		LER (secondary)& [\%] & 0$\pm$0 & 0 & 0 & 0 & 0 & 0 & 0\\\hline
		\end{tabular}}

		\caption{{\normalsize ULM distributions, measured with unmanaged nodes (policy 0). 
}}
		\vspace{10 mm}

		\resizebox{\textwidth}{!}{
		\begin{tabular}[t]{|l||c|c|c|c|c|c|c|c|}
		\hline ULM & unit & $ci_\mu$ & $s$ & min & $Q_1$ & $Q_2$ & $Q_3$ & max \\\hline
		ELT (primary)& [ms] & 445$\pm$6 & 19 & 425 & 431 & 438 & 458 & 501\\\hline
		NU (primary)& [MB/5 min] & 22$\pm$3 & 8 & 13 & 17 & 18 & 22 & 41\\\hline\hline
		LT (secondary)& [ms] & 445$\pm$2 & 152 & 86 & 354 & 445 & 552 & 2234\\\hline
		LET (secondary) & [ms]  & NA&  NA & NA & NA & NA & NA & NA  \\\hline
		LER (secondary)& [\%] & 0$\pm$0 & 0 & 0 & 0 & 0 & 0 & 0\\\hline
		\end{tabular}}

		\caption{{\normalsize ULM distributions, measured with managed nodes (policy 1). 
}}
		\vspace{10 mm}

		\resizebox{\textwidth}{!}{
		\begin{tabular}[t]{|l||c|c|c|c|c|c|c|c|}
		\hline ULM & unit & $ci_\mu$ & $s$ & min & $Q_1$ & $Q_2$ & $Q_3$ & max \\\hline
		ELT (primary)& [ms] & 428$\pm$4 & 12 & 394 & 421 & 430 & 436 & 444\\\hline
		NU (primary)& [MB/5 min] & 16$\pm$2 & 5 & 8 & 14 & 15 & 16 & 27\\\hline\hline
		LT (secondary)& [ms] & 428$\pm$2 & 142 & 87 & 322 & 419 & 549 & 1895\\\hline
		LET (secondary)& [ms] & 206$\pm$0 & 0 & 206 & 206 & 206 & 206 & 206\\\hline
		LER (secondary)& [\%] & 0$\pm$0 & 0 & 0 & 0 & 0 & 0 & 0\\\hline
		\end{tabular}}

		\caption{{\normalsize ULM distributions, measured with managed nodes (policy 2). 
}}
	\end{center}
\end{table}
\newpage

\subsection{\label{appendix::p2p:WL2_NB2}Synthetic Heavy Weight Workload with High Churn}

\subsubsection{Summarised Effects of Policies on Expected Lookup Time and Network Usage}
\begin{figure}[htpb]
	\centerline{{\resizebox{95mm}{!}{\includegraphics{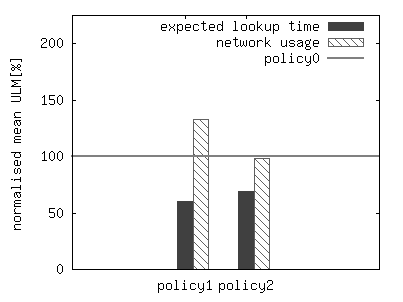}}}}
	\caption{\label{fig:Synthetic Heavy Weight Workload with High Churn user-level metrics} normalised mean ULM values}
\end{figure}
		\vspace{5 mm}

\begin{table}[htpb]
	\begin{center}
		\begin{tabular}[t]{|l|r|r|}
		\hline policy & mean expected lookup time [ms] & mean network usage [MB/5 min]  \\\hline
		 policy 0 &  727 & 25\\\hline
		 policy 1 & 440 & 33\\\hline
		 policy 2 & 504 & 24\\\hline
		\end{tabular}

		\caption{\label{tab:ULMWL2_NB2} mean ULM values}
	\end{center}
	\end{table}
\newpage

\subsubsection{Summary of ULM Distributions}
\begin{table}[htpb]
	\begin{center}
		\vspace{10 mm}

		\resizebox{\textwidth}{!}{
		\begin{tabular}[t]{|l||c|c|c|c|c|c|c|c|}
		\hline ULM & unit & $ci_\mu$ & $s$ & min & $Q_1$ & $Q_2$ & $Q_3$ & max \\\hline
		ELT (primary)& [ms] & 727$\pm$71 & 229 & 476 & 509 & 713 & 927 & 1168\\\hline
		NU (primary)& [MB/5 min] & 25$\pm$7 & 23 & 1 & 2 & 22 & 47 & 50\\\hline\hline
		LT (secondary)& [ms] & 590$\pm$4 & 256 & 97 & 406 & 623 & 750 & 4102\\\hline
		LET (secondary)& [ms] & 152$\pm$25 & 1181 & 6 & 67 & 99 & 110 & 45045\\\hline
		LER (secondary)& [\%] & 26$\pm$9 & 29 & 1 & 3 & 18 & 37 & 86\\\hline
		\end{tabular}}

		\caption{{\normalsize ULM distributions, measured with unmanaged nodes (policy 0). 
}}
		\vspace{10 mm}

		\resizebox{\textwidth}{!}{
		\begin{tabular}[t]{|l||c|c|c|c|c|c|c|c|}
		\hline ULM & unit & $ci_\mu$ & $s$ & min & $Q_1$ & $Q_2$ & $Q_3$ & max \\\hline
		ELT (primary)& [ms] & 440$\pm$9 & 30 & 372 & 435 & 449 & 455 & 501\\\hline
		NU (primary)& [MB/5 min] & 33$\pm$2 & 6 & 13 & 33 & 34 & 36 & 38\\\hline\hline
		LT (secondary)& [ms] & 434$\pm$3 & 208 & 94 & 278 & 412 & 558 & 2336\\\hline
		LET (secondary)& [ms] & 196$\pm$10 & 160 & 6 & 86 & 185 & 263 & 1506\\\hline
		LER (secondary)& [\%] & 4$\pm$0 & 2 & 1 & 3 & 3 & 4 & 7\\\hline
		\end{tabular}}

		\caption{{\normalsize ULM distributions, measured with managed nodes (policy 1). 
}}
		\vspace{10 mm}

		\resizebox{\textwidth}{!}{
		\begin{tabular}[t]{|l||c|c|c|c|c|c|c|c|}
		\hline ULM & unit & $ci_\mu$ & $s$ & min & $Q_1$ & $Q_2$ & $Q_3$ & max \\\hline
		ELT (primary)& [ms] & 504$\pm$66 & 210 & 332 & 411 & 422 & 522 & 1071\\\hline
		NU (primary)& [MB/5 min] & 24$\pm$2 & 7 & 4 & 24 & 26 & 28 & 33\\\hline\hline
		LT (secondary)& [ms] & 409$\pm$3 & 198 & 85 & 275 & 389 & 523 & 3555\\\hline
		LET (secondary)& [ms] & 482$\pm$247 & 6545 & 6 & 142 & 185 & 251 & 165072\\\hline
		LER (secondary)& [\%] & 11$\pm$3 & 10 & 5 & 7 & 8 & 11 & 56\\\hline
		\end{tabular}}

		\caption{{\normalsize ULM distributions, measured with managed nodes (policy 2). 
}}
	\end{center}
\end{table}
\newpage

\subsection{\label{appendix::p2p:WL2_NB3}Synthetic Heavy Weight Workload with Locally Varying Churn}

\subsubsection{Summarised Effects of Policies on Expected Lookup Time and Network Usage}
\begin{figure}[htpb]
	\centerline{{\resizebox{95mm}{!}{\includegraphics{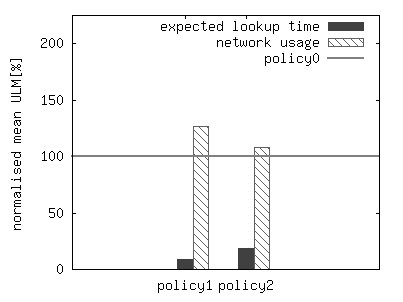}}}}
	\caption{\label{fig:Synthetic Heavy Weight Workload with Locally Varying Churn user-level metrics} normalised mean ULM values}
\end{figure}
		\vspace{5 mm}

\begin{table}[htpb]
	\begin{center}
		\begin{tabular}[t]{|l|r|r|}
		\hline policy & mean expected lookup time [ms] & mean network usage [MB/5 min]  \\\hline
		 policy 0 &  6495 & 23\\\hline
		 policy 1 & 552 & 30\\\hline
		 policy 2 & 1190 & 25\\\hline
		\end{tabular}

		\caption{\label{tab:ULMWL2_NB3} mean ULM values}
	\end{center}
	\end{table}
\newpage

\subsubsection{Summary of ULM Distributions}
\begin{table}[htpb]
	\begin{center}
		\vspace{10 mm}

		\resizebox{\textwidth}{!}{
		\begin{tabular}[t]{|l||c|c|c|c|c|c|c|c|}
		\hline ULM & unit & $ci_\mu$ & $s$ & min & $Q_1$ & $Q_2$ & $Q_3$ & max \\\hline
		ELT (primary)& [ms] & 6495$\pm$3107 & 15574 & 390 & 576 & 2120 & 8655 & 126505\\\hline
		NU (primary)& [MB/5 min] & 23$\pm$4 & 21 & 0 & 6 & 13 & 51 & 57\\\hline\hline
		LT (secondary)& [ms] & 840$\pm$9 & 657 & 98 & 416 & 647 & 944 & 6366\\\hline
		LET (secondary)& [ms] & 2447$\pm$531 & 17738 & 6 & 74 & 166 & 525 & 239475\\\hline
		LER (secondary)& [\%] & 33$\pm$5 & 24 & 0 & 2 & 43 & 53 & 69\\\hline
		\end{tabular}}

		\caption{{\normalsize ULM distributions, measured with unmanaged nodes (policy 0). 
}}
		\vspace{10 mm}

		\resizebox{\textwidth}{!}{
		\begin{tabular}[t]{|l||c|c|c|c|c|c|c|c|}
		\hline ULM & unit & $ci_\mu$ & $s$ & min & $Q_1$ & $Q_2$ & $Q_3$ & max \\\hline
		ELT (primary)& [ms] & 552$\pm$117 & 389 & 375 & 438 & 460 & 474 & 2522\\\hline
		NU (primary)& [MB/5 min] & 30$\pm$3 & 8 & 1 & 27 & 32 & 34 & 39\\\hline\hline
		LT (secondary)& [ms] & 444$\pm$3 & 204 & 84 & 279 & 421 & 589 & 2545\\\hline
		LET (secondary)& [ms] & 871$\pm$639 & 12153 & 6 & 143 & 186 & 236 & 251373\\\hline
		LER (secondary)& [\%] & 5$\pm$1 & 3 & 0 & 3 & 6 & 7 & 13\\\hline
		\end{tabular}}

		\caption{{\normalsize ULM distributions, measured with managed nodes (policy 1). 
}}
		\vspace{10 mm}

		\resizebox{\textwidth}{!}{
		\begin{tabular}[t]{|l||c|c|c|c|c|c|c|c|}
		\hline ULM & unit & $ci_\mu$ & $s$ & min & $Q_1$ & $Q_2$ & $Q_3$ & max \\\hline
		ELT (primary)& [ms] & 1190$\pm$325 & 1282 & 438 & 536 & 986 & 1268 & 7995\\\hline
		NU (primary)& [MB/5 min] & 25$\pm$2 & 9 & 5 & 17 & 27 & 33 & 42\\\hline\hline
		LT (secondary)& [ms] & 541$\pm$6 & 438 & 93 & 283 & 444 & 662 & 4759\\\hline
		LET (secondary)& [ms] & 1527$\pm$473 & 15181 & 6 & 141 & 186 & 243 & 239224\\\hline
		LER (secondary)& [\%] & 18$\pm$4 & 15 & 0 & 8 & 11 & 35 & 59\\\hline
		\end{tabular}}

		\caption{{\normalsize ULM distributions, measured with managed nodes (policy 2). 
}}
	\end{center}
\end{table}
\newpage

\subsection{\label{appendix::p2p:WL2_NB4}Synthetic Heavy Weight Workload with Temporally Varying Churn}

\subsubsection{Summarised Effects of Policies on Expected Lookup Time and Network Usage}
\begin{figure}[htpb]
	\centerline{{\resizebox{95mm}{!}{\includegraphics{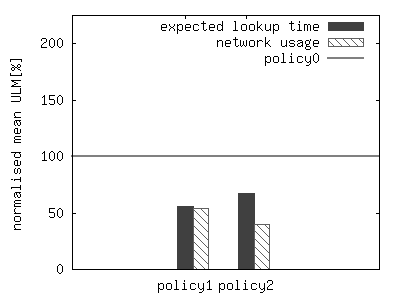}}}}
	\caption{\label{fig:Synthetic Heavy Weight Workload with Temporally Varying Churn user-level metrics} normalised mean ULM values}
\end{figure}
		\vspace{5 mm}

\begin{table}[htpb]
	\begin{center}
		\begin{tabular}[t]{|l|r|r|}
		\hline policy & mean expected lookup time [ms] & mean network usage [MB/5 min]  \\\hline
		 policy 0 &  804 & 51\\\hline
		 policy 1 & 452 & 28\\\hline
		 policy 2 & 540 & 20\\\hline
		\end{tabular}

		\caption{\label{tab:ULMWL2_NB4} mean ULM values}
	\end{center}
	\end{table}
\newpage

\subsubsection{Summary of ULM Distributions}
\begin{table}[htpb]
	\begin{center}
		\vspace{10 mm}

		\resizebox{\textwidth}{!}{
		\begin{tabular}[t]{|l||c|c|c|c|c|c|c|c|}
		\hline ULM & unit & $ci_\mu$ & $s$ & min & $Q_1$ & $Q_2$ & $Q_3$ & max \\\hline
		ELT (primary)& [ms] & 804$\pm$172 & 629 & 519 & 545 & 579 & 628 & 2684\\\hline
		NU (primary)& [MB/5 min] & 51$\pm$5 & 19 & 0 & 45 & 53 & 68 & 74\\\hline\hline
		LT (secondary)& [ms] & 622$\pm$5 & 408 & 98 & 409 & 570 & 739 & 6912\\\hline
		LET (secondary)& [ms] & 196$\pm$27 & 745 & 7 & 97 & 105 & 128 & 30077\\\hline
		LER (secondary)& [\%] & 10$\pm$6 & 24 & 0 & 0 & 1 & 5 & 100\\\hline
		\end{tabular}}

		\caption{{\normalsize ULM distributions, measured with unmanaged nodes (policy 0). 
}}
		\vspace{10 mm}

		\resizebox{\textwidth}{!}{
		\begin{tabular}[t]{|l||c|c|c|c|c|c|c|c|}
		\hline ULM & unit & $ci_\mu$ & $s$ & min & $Q_1$ & $Q_2$ & $Q_3$ & max \\\hline
		ELT (primary)& [ms] & 452$\pm$41 & 131 & 161 & 417 & 438 & 466 & 1030\\\hline
		NU (primary)& [MB/5 min] & 28$\pm$3 & 9 & 8 & 22 & 29 & 35 & 40\\\hline\hline
		LT (secondary)& [ms] & 418$\pm$3 & 198 & 85 & 276 & 412 & 543 & 2662\\\hline
		LET (secondary)& [ms] & 411$\pm$343 & 6669 & 6 & 177 & 184 & 231 & 213399\\\hline
		LER (secondary)& [\%] & 5$\pm$2 & 6 & 0 & 0 & 3 & 11 & 19\\\hline
		\end{tabular}}

		\caption{{\normalsize ULM distributions, measured with managed nodes (policy 1). 
}}
		\vspace{10 mm}

		\resizebox{\textwidth}{!}{
		\begin{tabular}[t]{|l||c|c|c|c|c|c|c|c|}
		\hline ULM & unit & $ci_\mu$ & $s$ & min & $Q_1$ & $Q_2$ & $Q_3$ & max \\\hline
		ELT (primary)& [ms] & 540$\pm$58 & 195 & 321 & 435 & 445 & 578 & 1088\\\hline
		NU (primary)& [MB/5 min] & 20$\pm$2 & 7 & 0 & 16 & 20 & 27 & 31\\\hline\hline
		LT (secondary)& [ms] & 444$\pm$2 & 185 & 85 & 304 & 425 & 560 & 2335\\\hline
		LET (secondary)& [ms] & 916$\pm$571 & 12514 & 6 & 179 & 185 & 233 & 246854\\\hline
		LER (secondary)& [\%] & 7$\pm$3 & 11 & 0 & 0 & 1 & 7 & 32\\\hline
		\end{tabular}}

		\caption{{\normalsize ULM distributions, measured with managed nodes (policy 2). 
}}
	\end{center}
\end{table}
\newpage

\subsection{\label{appendix::p2p:WL3_NB1}Synthetic Variabale Weight Workload with Low Churn}

\subsubsection{Summarised Effects of Policies on Expected Lookup Time and Network Usage}
\begin{figure}[htpb]
	\centerline{{\resizebox{95mm}{!}{\includegraphics{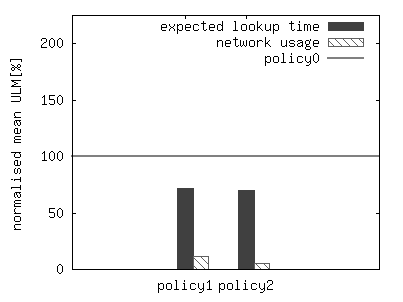}}}}
	\caption{\label{fig:Synthetic Variabale Weight Workload with Low Churn user-level metrics} normalised mean ULM values}
\end{figure}
		\vspace{5 mm}

\begin{table}[htpb]
	\begin{center}
		\begin{tabular}[t]{|l|r|r|}
		\hline policy & mean expected lookup time [ms] & mean network usage [MB/5 min]  \\\hline
		 policy 0 &  636 & 63\\\hline
		 policy 1 & 454 & 7\\\hline
		 policy 2 & 445 & 3\\\hline
		\end{tabular}

		\caption{\label{tab:ULMWL3_NB1} mean ULM values}
	\end{center}
	\end{table}
\newpage

\subsubsection{Summary of ULM Distributions}
\begin{table}[htpb]
	\begin{center}
		\vspace{10 mm}

		\resizebox{\textwidth}{!}{
		\begin{tabular}[t]{|l||c|c|c|c|c|c|c|c|}
		\hline ULM & unit & $ci_\mu$ & $s$ & min & $Q_1$ & $Q_2$ & $Q_3$ & max \\\hline
		ELT (primary)& [ms] & 636$\pm$6 & 23 & 593 & 618 & 633 & 654 & 699\\\hline
		NU (primary)& [MB/5 min] & 63$\pm$4 & 16 & 8 & 67 & 68 & 68 & 69\\\hline\hline
		LT (secondary)& [ms] & 638$\pm$7 & 235 & 98 & 461 & 643 & 797 & 2315\\\hline
		LET (secondary) & [ms]  & NA&  NA & NA & NA & NA & NA & NA  \\\hline
		LER (secondary)& [\%] & 0$\pm$0 & 0 & 0 & 0 & 0 & 0 & 0\\\hline
		\end{tabular}}

		\caption{{\normalsize ULM distributions, measured with unmanaged nodes (policy 0). 
}}
		\vspace{10 mm}

		\resizebox{\textwidth}{!}{
		\begin{tabular}[t]{|l||c|c|c|c|c|c|c|c|}
		\hline ULM & unit & $ci_\mu$ & $s$ & min & $Q_1$ & $Q_2$ & $Q_3$ & max \\\hline
		ELT (primary)& [ms] & 454$\pm$7 & 24 & 426 & 437 & 451 & 462 & 525\\\hline
		NU (primary)& [MB/5 min] & 7$\pm$1 & 4 & 3 & 4 & 6 & 8 & 18\\\hline\hline
		LT (secondary)& [ms] & 454$\pm$5 & 152 & 97 & 366 & 455 & 565 & 1826\\\hline
		LET (secondary) & [ms]  & NA&  NA & NA & NA & NA & NA & NA  \\\hline
		LER (secondary)& [\%] & 0$\pm$0 & 0 & 0 & 0 & 0 & 0 & 0\\\hline
		\end{tabular}}

		\caption{{\normalsize ULM distributions, measured with managed nodes (policy 1). 
}}
		\vspace{10 mm}

		\resizebox{\textwidth}{!}{
		\begin{tabular}[t]{|l||c|c|c|c|c|c|c|c|}
		\hline ULM & unit & $ci_\mu$ & $s$ & min & $Q_1$ & $Q_2$ & $Q_3$ & max \\\hline
		ELT (primary)& [ms] & 445$\pm$4 & 14 & 425 & 435 & 446 & 456 & 472\\\hline
		NU (primary)& [MB/5 min] & 3$\pm$0 & 1 & 1 & 3 & 3 & 4 & 7\\\hline\hline
		LT (secondary)& [ms] & 445$\pm$4 & 142 & 95 & 363 & 452 & 554 & 1836\\\hline
		LET (secondary) & [ms]  & NA&  NA & NA & NA & NA & NA & NA  \\\hline
		LER (secondary)& [\%] & 0$\pm$0 & 0 & 0 & 0 & 0 & 0 & 0\\\hline
		\end{tabular}}

		\caption{{\normalsize ULM distributions, measured with managed nodes (policy 2). 
}}
	\end{center}
\end{table}
\newpage

\subsection{\label{appendix::p2p:WL3_NB2}Synthetic Variabale Weight Workload with High Churn}

\subsubsection{Summarised Effects of Policies on Expected Lookup Time and Network Usage}
\begin{figure}[htpb]
	\centerline{{\resizebox{95mm}{!}{\includegraphics{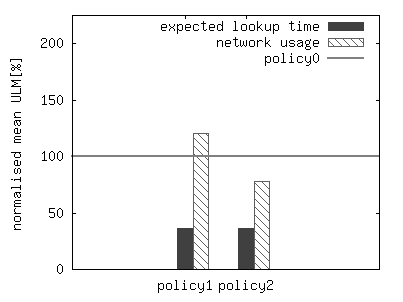}}}}
	\caption{\label{fig:Synthetic Variabale Weight Workload with High Churn user-level metrics} normalised mean ULM values}
\end{figure}
		\vspace{5 mm}

\begin{table}[htpb]
	\begin{center}
		\begin{tabular}[t]{|l|r|r|}
		\hline policy & mean expected lookup time [ms] & mean network usage [MB/5 min]  \\\hline
		 policy 0 &  1134 & 17\\\hline
		 policy 1 & 410 & 21\\\hline
		 policy 2 & 413 & 13\\\hline
		\end{tabular}

		\caption{\label{tab:ULMWL3_NB2} mean ULM values}
	\end{center}
	\end{table}
\newpage

\subsubsection{Summary of ULM Distributions}
\begin{table}[htpb]
	\begin{center}
		\vspace{10 mm}

		\resizebox{\textwidth}{!}{
		\begin{tabular}[t]{|l||c|c|c|c|c|c|c|c|}
		\hline ULM & unit & $ci_\mu$ & $s$ & min & $Q_1$ & $Q_2$ & $Q_3$ & max \\\hline
		ELT (primary)& [ms] & 1134$\pm$469 & 1611 & 464 & 550 & 838 & 986 & 9665\\\hline
		NU (primary)& [MB/5 min] & 17$\pm$6 & 19 & 0 & 0 & 4 & 38 & 45\\\hline\hline
		LT (secondary)& [ms] & 566$\pm$12 & 277 & 98 & 373 & 555 & 722 & 2535\\\hline
		LET (secondary)& [ms] & 243$\pm$152 & 3572 & 8 & 97 & 102 & 107 & 132041\\\hline
		LER (secondary)& [\%] & 50$\pm$12 & 42 & 0 & 1 & 84 & 86 & 90\\\hline
		\end{tabular}}

		\caption{{\normalsize ULM distributions, measured with unmanaged nodes (policy 0). 
}}
		\vspace{10 mm}

		\resizebox{\textwidth}{!}{
		\begin{tabular}[t]{|l||c|c|c|c|c|c|c|c|}
		\hline ULM & unit & $ci_\mu$ & $s$ & min & $Q_1$ & $Q_2$ & $Q_3$ & max \\\hline
		ELT (primary)& [ms] & 410$\pm$22 & 78 & 278 & 338 & 418 & 459 & 559\\\hline
		NU (primary)& [MB/5 min] & 21$\pm$2 & 7 & 0 & 19 & 23 & 25 & 27\\\hline\hline
		LT (secondary)& [ms] & 405$\pm$6 & 194 & 97 & 274 & 371 & 519 & 1977\\\hline
		LET (secondary)& [ms] & 122$\pm$10 & 105 & 6 & 85 & 87 & 144 & 633\\\hline
		LER (secondary)& [\%] & 9$\pm$6 & 20 & 0 & 1 & 2 & 8 & 86\\\hline
		\end{tabular}}

		\caption{{\normalsize ULM distributions, measured with managed nodes (policy 1). 
}}
		\vspace{10 mm}

		\resizebox{\textwidth}{!}{
		\begin{tabular}[t]{|l||c|c|c|c|c|c|c|c|}
		\hline ULM & unit & $ci_\mu$ & $s$ & min & $Q_1$ & $Q_2$ & $Q_3$ & max \\\hline
		ELT (primary)& [ms] & 413$\pm$35 & 123 & 128 & 314 & 423 & 497 & 628\\\hline
		NU (primary)& [MB/5 min] & 13$\pm$2 & 6 & 0 & 11 & 14 & 17 & 24\\\hline\hline
		LT (secondary)& [ms] & 389$\pm$7 & 202 & 89 & 244 & 354 & 506 & 2047\\\hline
		LET (secondary)& [ms] & 174$\pm$9 & 106 & 6 & 86 & 183 & 233 & 576\\\hline
		LER (secondary)& [\%] & 13$\pm$6 & 20 & 0 & 1 & 6 & 15 & 86\\\hline
		\end{tabular}}

		\caption{{\normalsize ULM distributions, measured with managed nodes (policy 2). 
}}
	\end{center}
\end{table}
\newpage

\subsection{\label{appendix::p2p:WL3_NB3}Synthetic Variabale Weight Workload with Locally Varying Churn}

\subsubsection{Summarised Effects of Policies on Expected Lookup Time and Network Usage}
\begin{figure}[htpb]
	\centerline{{\resizebox{95mm}{!}{\includegraphics{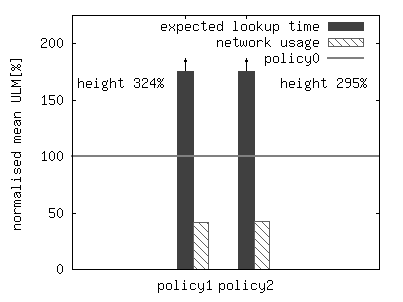}}}}
	\caption{\label{fig:Synthetic Variabale Weight Workload with Locally Varying Churn user-level metrics} normalised mean ULM values}
\end{figure}
		\vspace{5 mm}

\begin{table}[htpb]
	\begin{center}
		\begin{tabular}[t]{|l|r|r|}
		\hline policy & mean expected lookup time [ms] & mean network usage [MB/5 min]  \\\hline
		 policy 0 &  574 & 45\\\hline
		 policy 1 & 1858 & 19\\\hline
		 policy 2 & 1695 & 19\\\hline
		\end{tabular}

		\caption{\label{tab:ULMWL3_NB3} mean ULM values}
	\end{center}
	\end{table}
\newpage

\subsubsection{Summary of ULM Distributions}
\begin{table}[htpb]
	\begin{center}
		\vspace{10 mm}

		\resizebox{\textwidth}{!}{
		\begin{tabular}[t]{|l||c|c|c|c|c|c|c|c|}
		\hline ULM & unit & $ci_\mu$ & $s$ & min & $Q_1$ & $Q_2$ & $Q_3$ & max \\\hline
		ELT (primary)& [ms] & 574$\pm$28 & 97 & 367 & 535 & 574 & 601 & 1021\\\hline
		NU (primary)& [MB/5 min] & 45$\pm$1 & 3 & 37 & 43 & 45 & 47 & 50\\\hline\hline
		LT (secondary)& [ms] & 570$\pm$8 & 267 & 98 & 367 & 551 & 758 & 2096\\\hline
		LET (secondary)& [ms] & 966$\pm$262 & 1021 & 11 & 195 & 389 & 1726 & 4901\\\hline
		LER (secondary)& [\%] & 1$\pm$1 & 3 & 0 & 0 & 0 & 1 & 19\\\hline
		\end{tabular}}

		\caption{{\normalsize ULM distributions, measured with unmanaged nodes (policy 0). 
}}
		\vspace{10 mm}

		\resizebox{\textwidth}{!}{
		\begin{tabular}[t]{|l||c|c|c|c|c|c|c|c|}
		\hline ULM & unit & $ci_\mu$ & $s$ & min & $Q_1$ & $Q_2$ & $Q_3$ & max \\\hline
		ELT (primary)& [ms] & 1858$\pm$1360 & 5031 & 356 & 431 & 460 & 512 & 29491\\\hline
		NU (primary)& [MB/5 min] & 19$\pm$1 & 5 & 2 & 17 & 19 & 22 & 25\\\hline\hline
		LT (secondary)& [ms] & 444$\pm$6 & 200 & 98 & 282 & 427 & 589 & 2169\\\hline
		LET (secondary)& [ms] & 6804$\pm$4396 & 34634 & 7 & 143 & 188 & 279 & 223616\\\hline
		LER (secondary)& [\%] & 7$\pm$3 & 11 & 0 & 0 & 2 & 9 & 42\\\hline
		\end{tabular}}

		\caption{{\normalsize ULM distributions, measured with managed nodes (policy 1). 
}}
		\vspace{10 mm}

		\resizebox{\textwidth}{!}{
		\begin{tabular}[t]{|l||c|c|c|c|c|c|c|c|}
		\hline ULM & unit & $ci_\mu$ & $s$ & min & $Q_1$ & $Q_2$ & $Q_3$ & max \\\hline
		ELT (primary)& [ms] & 1695$\pm$967 & 3575 & 369 & 490 & 612 & 1434 & 21953\\\hline
		NU (primary)& [MB/5 min] & 19$\pm$3 & 10 & 4 & 12 & 16 & 25 & 40\\\hline\hline
		LT (secondary)& [ms] & 572$\pm$16 & 477 & 99 & 279 & 470 & 673 & 3561\\\hline
		LET (secondary)& [ms] & 2413$\pm$1427 & 18462 & 6 & 52 & 183 & 239 & 198501\\\hline
		LER (secondary)& [\%] & 18$\pm$5 & 18 & 0 & 1 & 12 & 33 & 71\\\hline
		\end{tabular}}

		\caption{{\normalsize ULM distributions, measured with managed nodes (policy 2). 
}}
	\end{center}
\end{table}
\newpage

\subsection{\label{appendix::p2p:WL3_NB4}Synthetic Variabale Weight Workload with Temporally Varying Churn}

\subsubsection{Summarised Effects of Policies on Expected Lookup Time and Network Usage}
\begin{figure}[htpb]
	\centerline{{\resizebox{95mm}{!}{\includegraphics{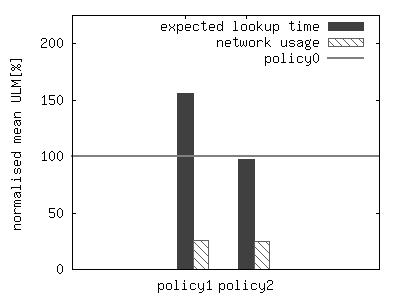}}}}
	\caption{\label{fig:Synthetic Variabale Weight Workload with Temporally Varying Churn user-level metrics} normalised mean ULM values}
\end{figure}
		\vspace{5 mm}

\begin{table}[htpb]
	\begin{center}
		\begin{tabular}[t]{|l|r|r|}
		\hline policy & mean expected lookup time [ms] & mean network usage [MB/5 min]  \\\hline
		 policy 0 &  570 & 52\\\hline
		 policy 1 & 889 & 13\\\hline
		 policy 2 & 555 & 13\\\hline
		\end{tabular}

		\caption{\label{tab:ULMWL3_NB4} mean ULM values}
	\end{center}
	\end{table}
\newpage

\subsubsection{Summary of ULM Distributions}
\begin{table}[htpb]
	\begin{center}
		\vspace{10 mm}

		\resizebox{\textwidth}{!}{
		\begin{tabular}[t]{|l||c|c|c|c|c|c|c|c|}
		\hline ULM & unit & $ci_\mu$ & $s$ & min & $Q_1$ & $Q_2$ & $Q_3$ & max \\\hline
		ELT (primary)& [ms] & 570$\pm$21 & 72 & 335 & 525 & 575 & 626 & 689\\\hline
		NU (primary)& [MB/5 min] & 52$\pm$3 & 10 & 40 & 45 & 47 & 63 & 68\\\hline\hline
		LT (secondary)& [ms] & 575$\pm$8 & 257 & 96 & 390 & 552 & 735 & 2111\\\hline
		LET (secondary)& [ms] & 162$\pm$56 & 144 & 14 & 49 & 143 & 231 & 495\\\hline
		LER (secondary)& [\%] & 1$\pm$0 & 1 & 0 & 0 & 0 & 1 & 5\\\hline
		\end{tabular}}

		\caption{{\normalsize ULM distributions, measured with unmanaged nodes (policy 0). 
}}
		\vspace{10 mm}

		\resizebox{\textwidth}{!}{
		\begin{tabular}[t]{|l||c|c|c|c|c|c|c|c|}
		\hline ULM & unit & $ci_\mu$ & $s$ & min & $Q_1$ & $Q_2$ & $Q_3$ & max \\\hline
		ELT (primary)& [ms] & 889$\pm$754 & 2633 & 149 & 386 & 444 & 489 & 15548\\\hline
		NU (primary)& [MB/5 min] & 13$\pm$2 & 7 & 0 & 10 & 13 & 19 & 24\\\hline\hline
		LT (secondary)& [ms] & 435$\pm$5 & 168 & 95 & 312 & 418 & 540 & 2148\\\hline
		LET (secondary)& [ms] & 8327$\pm$13486 & 103703 & 7 & 85 & 86 & 144 & 1311880\\\hline
		LER (secondary)& [\%] & 7$\pm$6 & 23 & 0 & 0 & 0 & 3 & 100\\\hline
		\end{tabular}}

		\caption{{\normalsize ULM distributions, measured with managed nodes (policy 1). 
}}
		\vspace{10 mm}

		\resizebox{\textwidth}{!}{
		\begin{tabular}[t]{|l||c|c|c|c|c|c|c|c|}
		\hline ULM & unit & $ci_\mu$ & $s$ & min & $Q_1$ & $Q_2$ & $Q_3$ & max \\\hline
		ELT (primary)& [ms] & 555$\pm$49 & 172 & 253 & 450 & 518 & 615 & 1162\\\hline
		NU (primary)& [MB/5 min] & 13$\pm$2 & 7 & 3 & 7 & 12 & 19 & 26\\\hline\hline
		LT (secondary)& [ms] & 479$\pm$6 & 186 & 96 & 362 & 461 & 588 & 2028\\\hline
		LET (secondary)& [ms] & 252$\pm$54 & 725 & 7 & 181 & 224 & 267 & 15926\\\hline
		LER (secondary)& [\%] & 15$\pm$6 & 21 & 0 & 0 & 1 & 28 & 77\\\hline
		\end{tabular}}

		\caption{{\normalsize ULM distributions, measured with managed nodes (policy 2). 
}}
	\end{center}
\end{table}
\newpage

\subsection{\label{appendix::p2p:WL4_NB1}File System Specific Workload with Low Churn}

\subsubsection{Summarised Effects of Policies on Expected Lookup Time and Network Usage}
\begin{figure}[htpb]
	\centerline{{\resizebox{95mm}{!}{\includegraphics{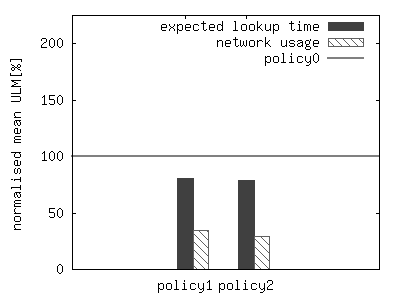}}}}
	\caption{\label{fig:File System Specific Workload with Low Churn user-level metrics} normalised mean ULM values}
\end{figure}
		\vspace{5 mm}

\begin{table}[htpb]
	\begin{center}
		\begin{tabular}[t]{|l|r|r|}
		\hline policy & mean expected lookup time [ms] & mean network usage [MB/5 min]  \\\hline
		 policy 0 &  877 & 76\\\hline
		 policy 1 & 705 & 26\\\hline
		 policy 2 & 690 & 22\\\hline
		\end{tabular}

		\caption{\label{tab:ULMWL4_NB1} mean ULM values}
	\end{center}
	\end{table}
\newpage

\subsubsection{Summary of ULM Distributions}
\begin{table}[htpb]
	\begin{center}
		\vspace{10 mm}

		\resizebox{\textwidth}{!}{
		\begin{tabular}[t]{|l||c|c|c|c|c|c|c|c|}
		\hline ULM & unit & $ci_\mu$ & $s$ & min & $Q_1$ & $Q_2$ & $Q_3$ & max \\\hline
		ELT (primary)& [ms] & 877$\pm$6 & 26 & 787 & 868 & 884 & 890 & 911\\\hline
		NU (primary)& [MB/5 min] & 76$\pm$2 & 11 & 21 & 79 & 79 & 80 & 81\\\hline\hline
		LT (secondary)& [ms] & 876$\pm$2 & 314 & 97 & 655 & 899 & 1110 & 2491\\\hline
		LET (secondary)& [ms] & 78$\pm$0 & 0 & 78 & 78 & 78 & 78 & 78\\\hline
		LER (secondary)& [\%] & 0$\pm$0 & 0 & 0 & 0 & 0 & 0 & 0\\\hline
		\end{tabular}}

		\caption{{\normalsize ULM distributions, measured with unmanaged nodes (policy 0). 
}}
		\vspace{10 mm}

		\resizebox{\textwidth}{!}{
		\begin{tabular}[t]{|l||c|c|c|c|c|c|c|c|}
		\hline ULM & unit & $ci_\mu$ & $s$ & min & $Q_1$ & $Q_2$ & $Q_3$ & max \\\hline
		ELT (primary)& [ms] & 705$\pm$3 & 14 & 684 & 694 & 699 & 714 & 732\\\hline
		NU (primary)& [MB/5 min] & 26$\pm$2 & 8 & 7 & 23 & 24 & 27 & 48\\\hline\hline
		LT (secondary)& [ms] & 705$\pm$2 & 244 & 96 & 541 & 742 & 899 & 2546\\\hline
		LET (secondary) & [ms]  & NA&  NA & NA & NA & NA & NA & NA  \\\hline
		LER (secondary)& [\%] & 0$\pm$0 & 0 & 0 & 0 & 0 & 0 & 0\\\hline
		\end{tabular}}

		\caption{{\normalsize ULM distributions, measured with managed nodes (policy 1). 
}}
		\vspace{10 mm}

		\resizebox{\textwidth}{!}{
		\begin{tabular}[t]{|l||c|c|c|c|c|c|c|c|}
		\hline ULM & unit & $ci_\mu$ & $s$ & min & $Q_1$ & $Q_2$ & $Q_3$ & max \\\hline
		ELT (primary)& [ms] & 690$\pm$6 & 25 & 603 & 685 & 695 & 704 & 727\\\hline
		NU (primary)& [MB/5 min] & 22$\pm$1 & 5 & 2 & 22 & 22 & 23 & 34\\\hline\hline
		LT (secondary)& [ms] & 690$\pm$2 & 238 & 93 & 530 & 726 & 887 & 2008\\\hline
		LET (secondary) & [ms]  & NA&  NA & NA & NA & NA & NA & NA  \\\hline
		LER (secondary)& [\%] & 0$\pm$0 & 0 & 0 & 0 & 0 & 0 & 0\\\hline
		\end{tabular}}

		\caption{{\normalsize ULM distributions, measured with managed nodes (policy 2). 
}}
	\end{center}
\end{table}
\newpage

\subsection{\label{appendix::p2p:WL4_NB2}File System Specific Workload with High Churn}

\subsubsection{Summarised Effects of Policies on Expected Lookup Time and Network Usage}
\begin{figure}[htpb]
	\centerline{{\resizebox{95mm}{!}{\includegraphics{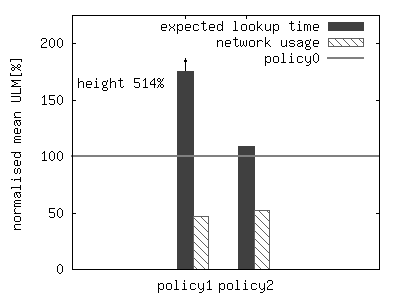}}}}
	\caption{\label{fig:File System Specific Workload with High Churn user-level metrics} normalised mean ULM values}
\end{figure}
		\vspace{5 mm}

\begin{table}[htpb]
	\begin{center}
		\begin{tabular}[t]{|l|r|r|}
		\hline policy & mean expected lookup time [ms] & mean network usage [MB/5 min]  \\\hline
		 policy 0 &  720 & 45\\\hline
		 policy 1 & 3704 & 21\\\hline
		 policy 2 & 784 & 23\\\hline
		\end{tabular}

		\caption{\label{tab:ULMWL4_NB2} mean ULM values}
	\end{center}
	\end{table}
\newpage

\subsubsection{Summary of ULM Distributions}
\begin{table}[htpb]
	\begin{center}
		\vspace{10 mm}

		\resizebox{\textwidth}{!}{
		\begin{tabular}[t]{|l||c|c|c|c|c|c|c|c|}
		\hline ULM & unit & $ci_\mu$ & $s$ & min & $Q_1$ & $Q_2$ & $Q_3$ & max \\\hline
		ELT (primary)& [ms] & 720$\pm$26 & 97 & 426 & 699 & 734 & 758 & 1003\\\hline
		NU (primary)& [MB/5 min] & 45$\pm$4 & 15 & 2 & 45 & 50 & 52 & 58\\\hline\hline
		LT (secondary)& [ms] & 726$\pm$3 & 341 & 86 & 506 & 715 & 934 & 6065\\\hline
		LET (secondary)& [ms] & 129$\pm$5 & 341 & 6 & 64 & 89 & 126 & 21026\\\hline
		LER (secondary)& [\%] & 10$\pm$7 & 25 & 0 & 2 & 3 & 4 & 97\\\hline
		\end{tabular}}

		\caption{{\normalsize ULM distributions, measured with unmanaged nodes (policy 0). 
}}
		\vspace{10 mm}

		\resizebox{\textwidth}{!}{
		\begin{tabular}[t]{|l||c|c|c|c|c|c|c|c|}
		\hline ULM & unit & $ci_\mu$ & $s$ & min & $Q_1$ & $Q_2$ & $Q_3$ & max \\\hline
		ELT (primary)& [ms] & 3704$\pm$436 & 2528 & 455 & 688 & 4739 & 5327 & 14954\\\hline
		NU (primary)& [MB/5 min] & 21$\pm$2 & 11 & 0 & 15 & 20 & 24 & 45\\\hline\hline
		LT (secondary)& [ms] & 1497$\pm$16 & 1970 & 97 & 506 & 732 & 1092 & 17915\\\hline
		LET (secondary)& [ms] & 3736$\pm$4763 & 205918 & 6 & 80 & 142 & 375 & 14630025\\\hline
		LER (secondary)& [\%] & 8$\pm$2 & 17 & 0 & 0 & 3 & 7 & 92\\\hline
		\end{tabular}}

		\caption{{\normalsize ULM distributions, measured with managed nodes (policy 1). 
}}
		\vspace{10 mm}

		\resizebox{\textwidth}{!}{
		\begin{tabular}[t]{|l||c|c|c|c|c|c|c|c|}
		\hline ULM & unit & $ci_\mu$ & $s$ & min & $Q_1$ & $Q_2$ & $Q_3$ & max \\\hline
		ELT (primary)& [ms] & 784$\pm$73 & 263 & 468 & 642 & 658 & 967 & 1688\\\hline
		NU (primary)& [MB/5 min] & 23$\pm$3 & 12 & 0 & 16 & 30 & 32 & 35\\\hline\hline
		LT (secondary)& [ms] & 609$\pm$3 & 271 & 86 & 418 & 616 & 781 & 5744\\\hline
		LET (secondary)& [ms] & 230$\pm$43 & 3153 & 6 & 72 & 118 & 183 & 244865\\\hline
		LER (secondary)& [\%] & 26$\pm$9 & 32 & 1 & 6 & 10 & 19 & 90\\\hline
		\end{tabular}}

		\caption{{\normalsize ULM distributions, measured with managed nodes (policy 2). 
}}
	\end{center}
\end{table}
\newpage

\subsection{\label{appendix::p2p:WL4_NB3}File System Specific Workload with Locally Varying Churn}

\subsubsection{Summarised Effects of Policies on Expected Lookup Time and Network Usage}
\begin{figure}[htpb]
	\centerline{{\resizebox{95mm}{!}{\includegraphics{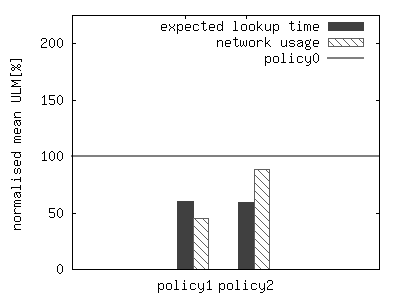}}}}
	\caption{\label{fig:File System Specific Workload with Locally Varying Churn user-level metrics} normalised mean ULM values}
\end{figure}
		\vspace{5 mm}

\begin{table}[htpb]
	\begin{center}
		\begin{tabular}[t]{|l|r|r|}
		\hline policy & mean expected lookup time [ms] & mean network usage [MB/5 min]  \\\hline
		 policy 0 &  6511 & 30\\\hline
		 policy 1 & 3908 & 13\\\hline
		 policy 2 & 3854 & 26\\\hline
		\end{tabular}

		\caption{\label{tab:ULMWL4_NB3} mean ULM values}
	\end{center}
	\end{table}
\newpage

\subsubsection{Summary of ULM Distributions}
\begin{table}[htpb]
	\begin{center}
		\vspace{10 mm}

		\resizebox{\textwidth}{!}{
		\begin{tabular}[t]{|l||c|c|c|c|c|c|c|c|}
		\hline ULM & unit & $ci_\mu$ & $s$ & min & $Q_1$ & $Q_2$ & $Q_3$ & max \\\hline
		ELT (primary)& [ms] & 6511$\pm$1001 & 8254 & 694 & 1431 & 4700 & 6031 & 52998\\\hline
		NU (primary)& [MB/5 min] & 30$\pm$2 & 13 & 5 & 18 & 30 & 38 & 61\\\hline\hline
		LT (secondary)& [ms] & 1821$\pm$16 & 1991 & 98 & 591 & 925 & 2479 & 22314\\\hline
		LET (secondary)& [ms] & 6117$\pm$781 & 28939 & 6 & 191 & 449 & 993 & 241662\\\hline
		LER (secondary)& [\%] & 18$\pm$2 & 18 & 0 & 3 & 6 & 37 & 68\\\hline
		\end{tabular}}

		\caption{{\normalsize ULM distributions, measured with unmanaged nodes (policy 0). 
}}
		\vspace{10 mm}

		\resizebox{\textwidth}{!}{
		\begin{tabular}[t]{|l||c|c|c|c|c|c|c|c|}
		\hline ULM & unit & $ci_\mu$ & $s$ & min & $Q_1$ & $Q_2$ & $Q_3$ & max \\\hline
		ELT (primary)& [ms] & 3908$\pm$398 & 2593 & 600 & 982 & 3866 & 5946 & 9414\\\hline
		NU (primary)& [MB/5 min] & 13$\pm$2 & 15 & 1 & 2 & 3 & 28 & 49\\\hline\hline
		LT (secondary)& [ms] & 1053$\pm$8 & 946 & 97 & 529 & 759 & 1051 & 6816\\\hline
		LET (secondary)& [ms] & 2027$\pm$260 & 15234 & 6 & 90 & 368 & 852 & 247382\\\hline
		LER (secondary)& [\%] & 37$\pm$3 & 22 & 0 & 10 & 51 & 55 & 60\\\hline
		\end{tabular}}

		\caption{{\normalsize ULM distributions, measured with managed nodes (policy 1). 
}}
		\vspace{10 mm}

		\resizebox{\textwidth}{!}{
		\begin{tabular}[t]{|l||c|c|c|c|c|c|c|c|}
		\hline ULM & unit & $ci_\mu$ & $s$ & min & $Q_1$ & $Q_2$ & $Q_3$ & max \\\hline
		ELT (primary)& [ms] & 3854$\pm$660 & 3971 & 525 & 818 & 2401 & 5529 & 21939\\\hline
		NU (primary)& [MB/5 min] & 26$\pm$2 & 10 & 10 & 18 & 24 & 35 & 49\\\hline\hline
		LT (secondary)& [ms] & 798$\pm$5 & 571 & 90 & 453 & 709 & 943 & 5477\\\hline
		LET (secondary)& [ms] & 2716$\pm$421 & 21396 & 6 & 99 & 360 & 562 & 274519\\\hline
		LER (secondary)& [\%] & 30$\pm$4 & 23 & 1 & 8 & 28 & 52 & 68\\\hline
		\end{tabular}}

		\caption{{\normalsize ULM distributions, measured with managed nodes (policy 2). 
}}
	\end{center}
\end{table}
\newpage

\subsection{\label{appendix::p2p:WL4_NB4}File System Specific Workload with Temporally Varying Churn}

\subsubsection{Summarised Effects of Policies on Expected Lookup Time and Network Usage}
\begin{figure}[htpb]
	\centerline{{\resizebox{95mm}{!}{\includegraphics{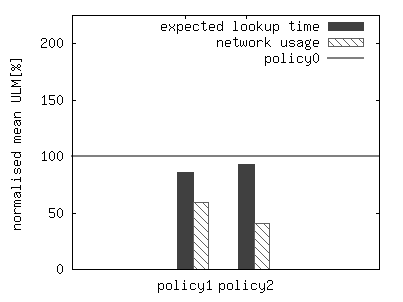}}}}
	\caption{\label{fig:File System Specific Workload with Temporally Varying Churn user-level metrics} normalised mean ULM values}
\end{figure}
		\vspace{5 mm}

\begin{table}[htpb]
	\begin{center}
		\begin{tabular}[t]{|l|r|r|}
		\hline policy & mean expected lookup time [ms] & mean network usage [MB/5 min]  \\\hline
		 policy 0 &  783 & 58\\\hline
		 policy 1 & 675 & 34\\\hline
		 policy 2 & 730 & 24\\\hline
		\end{tabular}

		\caption{\label{tab:ULMWL4_NB4} mean ULM values}
	\end{center}
	\end{table}
\newpage

\subsubsection{Summary of ULM Distributions}
\begin{table}[htpb]
	\begin{center}
		\vspace{10 mm}

		\resizebox{\textwidth}{!}{
		\begin{tabular}[t]{|l||c|c|c|c|c|c|c|c|}
		\hline ULM & unit & $ci_\mu$ & $s$ & min & $Q_1$ & $Q_2$ & $Q_3$ & max \\\hline
		ELT (primary)& [ms] & 783$\pm$17 & 69 & 467 & 743 & 777 & 841 & 876\\\hline
		NU (primary)& [MB/5 min] & 58$\pm$4 & 15 & 3 & 54 & 58 & 63 & 80\\\hline\hline
		LT (secondary)& [ms] & 770$\pm$3 & 322 & 86 & 551 & 783 & 1004 & 4684\\\hline
		LET (secondary)& [ms] & 114$\pm$6 & 232 & 5 & 47 & 54 & 73 & 8667\\\hline
		LER (secondary)& [\%] & 3$\pm$2 & 10 & 0 & 0 & 1 & 2 & 70\\\hline
		\end{tabular}}

		\caption{{\normalsize ULM distributions, measured with unmanaged nodes (policy 0). 
}}
		\vspace{10 mm}

		\resizebox{\textwidth}{!}{
		\begin{tabular}[t]{|l||c|c|c|c|c|c|c|c|}
		\hline ULM & unit & $ci_\mu$ & $s$ & min & $Q_1$ & $Q_2$ & $Q_3$ & max \\\hline
		ELT (primary)& [ms] & 675$\pm$14 & 55 & 496 & 636 & 690 & 713 & 791\\\hline
		NU (primary)& [MB/5 min] & 34$\pm$2 & 7 & 10 & 30 & 35 & 40 & 46\\\hline\hline
		LT (secondary)& [ms] & 654$\pm$2 & 263 & 86 & 471 & 669 & 842 & 2625\\\hline
		LET (secondary)& [ms] & 330$\pm$9 & 258 & 6 & 211 & 327 & 414 & 9940\\\hline
		LER (secondary)& [\%] & 5$\pm$1 & 5 & 0 & 0 & 3 & 7 & 18\\\hline
		\end{tabular}}

		\caption{{\normalsize ULM distributions, measured with managed nodes (policy 1). 
}}
		\vspace{10 mm}

		\resizebox{\textwidth}{!}{
		\begin{tabular}[t]{|l||c|c|c|c|c|c|c|c|}
		\hline ULM & unit & $ci_\mu$ & $s$ & min & $Q_1$ & $Q_2$ & $Q_3$ & max \\\hline
		ELT (primary)& [ms] & 730$\pm$85 & 335 & 272 & 570 & 681 & 754 & 2353\\\hline
		NU (primary)& [MB/5 min] & 24$\pm$2 & 9 & 0 & 20 & 25 & 29 & 41\\\hline\hline
		LT (secondary)& [ms] & 608$\pm$2 & 273 & 85 & 388 & 617 & 817 & 2724\\\hline
		LET (secondary)& [ms] & 1002$\pm$674 & 25285 & 6 & 145 & 282 & 381 & 1466637\\\hline
		LER (secondary)& [\%] & 9$\pm$3 & 14 & 0 & 0 & 2 & 10 & 60\\\hline
		\end{tabular}}

		\caption{{\normalsize ULM distributions, measured with managed nodes (policy 2). 
}}
	\end{center}
\end{table}
