# Supplementary material for: Autonomic Management in a Distributed Storage System
Source: arXiv:1007.0328 source file (2010-07-02)
Supplement: Supplementary file 18 [file p2p_main_results_stats_p.tex]

\subsection{\label{appendix::all_p_values}Analysis for Statistical Significance}

An analysis of the statistical significance of the differences between the data sets was carried out following guidelines for a \emph{t-test} from \cite{1991artofperformanceanalysis} and by using \emph{Commons-Math: The Apache Commons Mathematics Library}, commons-math 1.2, \cite{apache_commons_stats}.
The \emph{p-values}, shown in table \ref{tab:all_p} represent the probabilities that any differences in the monitored effects were only due to chance. 

\begin{table}[ht!]
\begin{center}
\begin{tabular}{|l|l||p{1.5cm}|p{1.5cm}||p{1.5cm}|p{1.5cm}|}
\hline
\multicolumn{2}{|c||}{experiment specification}&
\multicolumn{2}{c||}{policy 1}&
\multicolumn{2}{c|}{policy 2}\\\hline
\multicolumn{1}{|m{2cm}|}{workload}&
\multicolumn{1}{m{4cm}||}{churn pattern}&
\multicolumn{1}{m{1.5cm}|}{expected lookup time}&
\multicolumn{1}{m{1.5cm}||}{network usage}&
\multicolumn{1}{m{1.5cm}|}{expected lookup time}&
\multicolumn{1}{m{1.5cm}|}{network usage}\\\hline
%Synthetic Light Weight Workload Network with 
\multirow{4}{*}{\begin{sideways}synthetic\end{sideways}\begin{sideways}light\end{sideways} \begin{sideways}weight\end{sideways}} & low churn&0.000&0.000&0.000&0.000\\
& high churn&0.123&0.000&0.222&0.000\\
& locally varying churn&0.078&0.000&0.249&0.000\\
& temporally varying churn&0.027&0.000&0.903&0.000\\\hline
%Synthetic Heavy Weight Workload 
\multirow{4}{*}{\begin{sideways}synthetic\end{sideways}\begin{sideways}heavy\end{sideways} \begin{sideways}weight\end{sideways}} & low churn&0.000&0.000&0.000&0.000\\
& high churn&0.000&0.074&0.000&0.925\\
&locally varying churn&0.002&0.039&0.007&0.517\\
&temporally varying churn&0.002&0.000&0.022&0.000\\\hline
%Synthetic Varied Weight Workload                                               
\multirow{4}{*}{\begin{sideways}synthetic\end{sideways}\begin{sideways}variable\end{sideways} \begin{sideways}weight\end{sideways}}
& low churn&0.000&0.000&0.000&0.000\\
&high churn&0.016&0.341&0.017&0.297\\
&locally varying churn&0.129&0.000&0.065&0.000\\
&temporally varying churn&0.492&0.000&0.647&0.000\\\hline
%File System Workload 
\multirow{4}{*}{\begin{sideways}file\end{sideways} \begin{sideways}system\end{sideways}\begin{sideways}specific\end{sideways}}& low churn&0.000&0.000&0.000&0.000\\
&high churn&0.000&0.000&0.181&0.000\\
&locally varying churn&0.000&0.000&0.000&0.012\\
&temporally varying churn&0.000&0.000&0.318&0.000\\\hline
\end{tabular}
\caption{T-Test Results.}
\label{tab:all_p}
\end{center}
\end{table}
